# Supplementary material for: Max-Margin Token Selection in Attention Mechanism
Source: arXiv:2306.13596 source file (2023-12-08)
Supplement: Supplementary file 1 [file app_attempt.tex]

\section{Attempt at Gradient Flow Analysis (work in progress)}

\textbf{Counterexample:} Set $\ub=\X\vb=[1,0,0.99]$ and set keys $\Kb=[1,0,-10]$. Set $\pb=p$ to be a scalar. The loss function is simply
\[
-\Lc(p)=\ub^\top \sft{\Kb\pb}=[1,0,0.99]^\top \sft{[1,0,-10]p}=\frac{e^p+0.99e^{-10p}}{e^p+1+e^{-10p}}.
\]
GD will not work when started from init $p_0=-1$ (because it will eventually go to $p\rightarrow-\infty$ and achieve $-0.99$ loss).

On the other hand, best token is separable and optimal sol'n is $\infty\cdot \ps$ with $\ps=1$.

\begin{theorem}\label{lin flow thm} Consider the single input loss with label $Y=1$ and $\ell(y,\hat{y})=-y\hat{y}$
\begin{align}
\Lc(\pb)=-\vb^\top\X^\top \sft{\Kb\pb}.\label{one loss}
\end{align}
Fix a vector $\vb\in\R^d$ and define
\[
\alpha = \arg\max_{u\in [T]}\vb^\top \x_u,
\]
and suppose $\vb^\top (\x_{\alpha}-\x_u)>0$ for all $u\neq \alpha$. \eqref{one loss} with exponential loss and gradient flow $\dpb_t=-\nabla \Lc(\pb_t)$ converges (after normalization) to the \eqref{svm} solution
\[
\ps=\arg\min_{\pb} \tn{\pb}\quad \text{such that}\quad  \pb^\top(\kb_{\alpha}-\kb_{u\neq \alpha})\geq 1.
\]
\end{theorem}
\begin{proof} Set $\Sbt=\sft{\Kb\pb_t}$ and $\Sbtt=\sfp{\Kb\pb_t}$. Define $\gmax=\vb^\top\x_\alpha$ and $\ggap=\gmax-\max_{u\neq \alpha}\vb^\top\x_u$. Let us first write the gradient flow iterations
\[
\dpb_t=\X^\top \Sbtt\X\vb.%\cdot\exp(-\vb^\top \X^\top \Sbt).
\]
Here recall that $\sfp{\ab}=\diag{\sft{\ab}}-\sft{\ab}\sft{\ab}^\top$. Let us introduce the following notation
\begin{itemize}
\item $s_t=\sum_{u\neq \alpha}\Sbt_u$ (amount of irrelevance)
\item $\bgam=\X\vb$ (vector of scores)
\item $\obo=s_t^{-1}\sum_{u\neq \alpha}\Sbt_u\x_u$ (irrelevant mixture weighted by softmax)
\item $\agam=s_t^{-1}\sum_{u\neq \alpha}\bgam_u\Sbt_u$ (average score over irrelevant tokens).
\item $\obt=\agam^{-1}s_t^{-1}\sum_{u\neq \alpha}\bgam_u\Sbt_u\x_u$ (irrelevant mixture weighted by softmax and $\vb$)
\end{itemize}

With this notation, we can write
\begin{align}
\x(t)&:=\X^\top \Sbt=(1-s_t)\x_\alpha+s_t\obo\\
\xv(t)&:=\X^\top \diag{\Sbt}\X\vb=\gmax(1-s_t)\x_\alpha+\agam s_t\obt\\
\xw(t)&:=\X^\top \Sbt{\Sbt}^\top\X\vb=(\gmax(1-s_t)+\agam s_t)((1-s_t)\x_\alpha+s_t\obo)\\
\dpb_t&:=(1-s_t)s_t(\gmax-\agam)\x_\alpha+s_t[\agam \obt-(\gmax(1-s_t)+\agam s_t)\obo]
\end{align}
where $\dpb_t=\xv(t)-\xw(t)$. Note that $\dpb_t$ has strictly positive $\x_\alpha$ direction. In particular, $\dpb_t$ will be dominated by support vectors because $(1-s_t)s_t$ is maximized when $s_t$ is farther away from $0$ or $1$ (which happens at the support vectors).\vspace{20pt}

\textbf{Step 1:} Set $\pb'=\pb+\eps \ps$. $\db$ such that $\db^\top (\x_\alpha-\x_u)=1$ for all $u$. Claim that $\sft{\Kb\pb'}_\alpha > \sft{\Kb\pb}_\alpha$ and $\alpha$ increases.

\[
\frac{e^{x_u}}{\sum_{u\in[T]}e^{x_u}}\rightarrow\frac{e^{x_u}}{\sum_{u\neq\alpha}e^{x_u}+e^{x_\alpha+\eps}}.
\]
\textbf{Step 2:} If $\sft{\Kb\pb'}_\alpha > \sft{\Kb\pb}_\alpha$ and only $\alpha$ increases. Set $p_{\text{diff}}=\sft{\Kb\pb'}_\alpha - \sft{\Kb\pb}_\alpha$, then loss function improves by $p_{\text{diff}}\cdot \ggap$. Set $\bgam=\X\vb$. $p^{\text{rest}}_u=\sft{\Kb\pb'}_u-\sft{\Kb\pb}_u$.
%, $p^{\text{rest}}=\sum_{u\neq \alpha} p^{\text{rest}}_u$.
\begin{align} 
\Lc(\pb')-\Lc(\pb)&=-\sum_{u\in [T]}\bgam_u  (\sft{\Kb\pb'}_u-\sft{\Kb\pb}_u)= -p_{\text{diff}}\bgam_\alpha -\sum_{u\neq \alpha}\bgam_u p^{\text{rest}}_u\\
&\leq  -p_{\text{diff}}\bgam_\alpha +p^{\text{diff}}\max_{u\neq \alpha}\bgam_u\\
&\leq  -p_{\text{diff}}\ggap.
\end{align}

\%\%\%\%\%\%\%\%\%\%\%\% BREAK \%\%\%\%\%\%\%\%\%\%\%\%
\vspace{20pt}

%\newpage
%Also define $\xv(t)=\X^\top \diag{\sft{\Kb\pb_t}}\X\vb=\sum_{k\in [T]}\x_u$ and 
Now note that
\[
\X^\top \sfp{\Kb\pb_t}\X\vb=-\x(t)\x(t)^\top\vb
\]
\[
\dpb_t=\X^\top \sfp{\Kb\pb_t}\X\vb\cdot\exp(-\vb^\top \x(t)).
\]
We claim that $\pb_t=\log(t)\cdot\ps+\rb_t$ where $\rb_t$ will be a small (sub-logarithmic) residual. Let us write 
\begin{align}
\drb_t&=\X^\top \sfp{\Kb\pb_t}\X\vb-\frac{1}{t}\ps.
\end{align}
Observe that
\begin{align}
\sft{\Kb\pb_t}=\sft{\Kb(\log(t)\cdot\ps+\rb_t)}=
\end{align}
Let $\Kb'$ be the matrix with rows $\kb'_u=\kb_u-\kb_\alpha$. Set $\eb^t=\exp(\Kb'\pb_t)$.
\begin{align}
\eb^t_u=e^{-(\kb_\alpha-\kb_u)^\top \pb_t}=\begin{cases}1\quad\text{if}\quad u=\alpha\\t^{-1}e^{-\kb_u'^\top \rb_t}\quad\text{if}\quad u\in \supp\\ \leq t^{-\theta}e^{-\kb_u'^\top \rb_t} \quad u\in \supp^c\end{cases}
\end{align}
\end{proof}
