# Supplementary material for: Max-Margin Token Selection in Attention Mechanism
Source: arXiv:2306.13596 source file (2023-12-08)
Supplement: Supplementary file 2 [file app_local_path.tex]

\section{Analysis of the Local Regularization Path}

\subsection{Proof of Theorem~\ref{local path theorem}}

\begin{proof} We will prove that $\prl{R}$ is the optimal direction and also $\tn{\prl{R}}\rightarrow \infty$. 
    
\noindent\textbf{Step 1:} Let us first prove that $\prl{R}$ with $R\rightarrow\infty$ achieves the optimal risk. Thanks to $\prl{R}$ being the separator of tokens $\bal$, we have that
\begin{align*}
\lim_{R\rightarrow\infty}\Lc(\prl{R}) =\Lc_\star= \frac{1}{n}\sum_{i=1}^n\ell(\bgam_{i\alpha_i}).
\end{align*}
On the other hand, for any choice of $\pb\in \text{cone}(\bal)$, set $\x^\pb_i=\sum_{t=1}^T \sft{\Kb_i\pb}_t\x_t$. We can decompose it as
\begin{align}
\x^\pb_i=\sft{\Kb_i\pb}_{\alpha_i}\x_{i\alpha_i}+\sum_{t\in\Tc_i}\sft{\Kb_i\pb}_t\x_{it}+\sum_{t\in\Tcb_i}\sft{\Kb_i\pb}_t\x_{it}.
\end{align}
% and dropping subscript $i$
Setting $\ab_i=\Kb_i\pb$ and $\s_i=\sft{\ab_i}$. We can write the score as
\begin{align}\label{score decomp}
\bgam^\pb_i=\s_{\alpha_i}\bgam_{i\alpha_i}+\sum_{t\in\Tc_i}\s_t\bgam_{it}+\sum_{t\in\Tcb_i}\s_t\bgam_{it}.
\end{align}
Set $\bgg_{it}=\bgam_{it}-\bgam_{i\alpha_i}$ and let $A=\min_{t\in\Tc_i}-\bgg_{it}>0$ and $B=\max_{t\in\Tcb_i}\bgg_{it}$. Also let $P=\sum_{t\in\Tc_i}\s_{it}$ and $Q=\sum_{t\in\Tcb_i}\s_{it}$. Defining $\bgam^\pb_i=\vb^\top \x^\pb_i$, the score increment obeys given by
\[
\bgam^\pb_i-\bgam_{\alpha_i}=\sum_{t\in\Tc_i}\s_t\bgg_{it}+\sum_{t\in\Tcb_i}\s_t\bgg_{it}\leq BQ-AP.
\]
Now since $\pb\in \text{cone}(\bal)$, there exists $t\in \Tc_i$ obeying $\min_{\tau\in\Tcb_i}\pb^\top (\kb_{it}-\kb_{i\tau})=\ab_{it}-\ab_{i\tau}\geq \eps \tn{\pb}$. Let $D=(\sum_{t\in [T]}e^{\ab_{it}})^{-1}$. Consequently,
\[
Q=\sum_{\tau\in\Tcb_i}\s_{i\tau}=D\sum_{\tau\in\Tcb_i}e^{\ab_{i\tau}}\leq DTe^{\ab_{it}-\eps\tn{\pb}}\leq Te^{-\eps\tn{\pb}}P.
\]
Consequently,
\[
\bgam^\pb_i-\bgam_{\alpha_i}\leq BQ-AP\leq (BTe^{-\eps\tn{\pb}}-A)P.
\]
The right hand side is negative as soon as $\tn{\pb}\geq \Xi>\frac{1}{\eps}\log\frac{BT}{A}$ as desired and we conclude by strict-decreasing-ness of $\ell$.

\noindent\textbf{Step 2:} To proceed, we show that $\prl{R}$ converges in direction to $\ps$. As usual, suppose this is not the case and let us obtain a contradiction by showing that $\pst_R=R\cdot\ps/\tn{\ps}$. Also define $\prb{R}=R\cdot\prl{R}/\tn{\prl{R}}$. Since direction fails to converge, for some $\delta>0$, there exists arbitrarily large $R>0$ such that $\tn{\prb{R}-\ps}\geq \delta$. Alternatively, we can translate this to the suboptimality of the SVM. Namely, there exists an (updated) $\delta>0$ such that, $\prb{R}$ strictly violates at least one of the inequality constraints in \eqref{attnsvm}. Without losing generality, suppose $\prb{R}$ violates the first constraint, that is, for $i=1$ and some $\tau\in \Tc_1$, 
\[
\pb^\top(\kb_{i\alpha_1}-\kb_{i\tau})\leq 1-\delta. 
\]
Now, we will argue that this will lead to a contradiction by showing $\Lc(\pb^\st_R)<\Lc(\prl{R})$ for sufficiently large $R$.

To show the result, we establish a refined probability control as in Step 1 by studying distance to $\Lc_\star$. Denote $\bgam^R_i=\bgam_i^{\prl{R}}$ as shorthand. Let $\s_i^R=\sft{\ab^R}$ with $\ab_i^R=\Kb_i\prl{R}$. Set the corresponding notation for $\pst_R$ with $\bgam^\st,\s^\st,\ab^\st$. Set fixed scalars (independent of $\pb$ choices) $A_1=\bgam_{1\alpha_1}-\max_{t\in\Tc_1}\bgam_{1t}>0$ and $A_2=\bgam_{1\alpha_1}-\max_{t\in[T]}\bgam_{1t}$. 

Critically, recall the inequalities (regardless of $\prl{R}$ or $\pst_R$)
\[
Q=\sum_{\tau\in\Tcb_i}\s_{i\tau}=D\sum_{\tau\in\Tcb_i}e^{\ab_{i\tau}}\leq DTe^{\ab_{it}-\eps\tn{\pb}}\leq Te^{-\eps\tn{\pb}}P\leq Te^{-\eps\tn{\pb}}(1-\s_{\alpha_i})\quad\text{where}\quad P=\sum_{\tau\in\Tc_i}\s_{i\tau}\leq 1-\s_{\alpha_i}.
\]
Set $R'=\tn{\prl{R}}$. On top of this, we note the probability inequalities on the selected tokens $\alpha_i$
\[
\s^\st_{i\alpha_i}\geq 1-Te^{-R\Gamma}\quad \text{and}\quad s^R_{i\alpha_i}\leq \frac{1}{1+e^{-(1-\delta)R'\Gamma}}.
\]
The latter arises from the $\delta$-margin violation. Since $\ell$ is decreasing and scores are bounded (as $\vb$ is bounded), we know that $\ell'(\bgam^\pb)<0$ and $|\ell'(\bgam^\pb)|<C$ for some constant $C>0$. Denote $\ell'_R,\ell'_\st$ to be the derivative of $\ell(x)$ used for first-order Taylor expansion below. Thus, following \eqref{score decomp} and using we can write
\begin{align}
\Lc(\prl{R})-\Lc_\star&\geq \frac{1}{n}[\ell(\bgam_1^{\prl{R}})-\ell(\bgam_{\alpha_1})]\geq \frac{-\ell'_R}{n}(\bgam_{\alpha_1}-\bgam_1^{\prl{R}})\\
&\geq \frac{-\ell'_R}{n}(1-\s_{1\alpha_1}^R)(A_1+A_2Te^{-\eps R'})\\
&\geq \frac{-\ell'_R}{n}\frac{1}{1+e^{(1-\delta)R'\Gamma}}(A_1+A_2Te^{-\eps R'}).
%[\frac{A_1}{1+e^{(1-\delta)R'\Gamma}}+A_2Te^{-\eps R'}].
\end{align}
Above, recalling the choice $\Xi\geq O(1/\eps)$, $R'\geq \Xi$ implies $|A_2|Te^{-\eps R'}\leq A_1/2$ to obtain
\begin{align}
\Lc(\prl{R})-\Lc_\star\geq \frac{-\ell'_R\cdot A_1}{2n}\frac{1}{1+e^{(1-\delta)R'\Gamma}}\geq \frac{-\ell'_R\cdot A_1}{2n}\frac{1}{1+e^{(1-\delta)R\Gamma}}.\label{ineq prl}
\end{align}
Conversely, we upper bound the difference between $\Lc(\pst_R)$ and $\Lc_\star$ as follows. Define $B_1=\max_{i\in[n]}\{\bgam_{i\alpha_i}-\min_{t\in\Tc_1}\bgam_{it}\}>0$ and $B_2=\max_{i\in[n]}\{\bgam_{i\alpha_i}-\min_{t\in[T]}\bgam_{it}\}$. Let $j=\arg\max_{i\in[n]}[\ell(\bgam_i^{\pst_R})-\ell(\bgam_{\alpha_i})]$.
\begin{align}
\Lc(\pst_R)-\Lc_\star&\leq \max_{i\in[n]}[\ell(\bgam_i^{\pst_R})-\ell(\bgam_{\alpha_i})]\leq -\ell'_\st\cdot(\bgam_{\alpha_j}-\bgam_j^{\pst_R})\\
&\leq -\ell'_\st\cdot(1-\s_{1\alpha_j}^\st)(B_1+B_2Te^{-\eps R})\\
&\leq -\ell'_\st\cdot Te^{-R\Gamma}(B_1+B_2Te^{-\eps R})\\
&\leq -2\ell'_\st\cdot Te^{-R\Gamma}B_1,
\end{align}
where we again used the fact that $R\geq \Xi$ is large enough to ensure $B_2Te^{-\eps R}\leq B_1$.

Combining the last inequality and \eqref{ineq prl}, and using $\ell'_\st/\ell'_R<C$ for some constant $C>0$, we conclude that $\Lc(\pst_R)<\Lc(\prl{R})$ whenever
\[
2CT\cdot e^{-R\Gamma}B_1<\frac{A_1}{2n}\frac{1}{1+e^{(1-\delta)R\Gamma}}\iff \frac{e^{R\Gamma}}{1+e^{(1-\delta)R\Gamma}}> \frac{4CTn B_1}{A_1}.
\]
This holds for all $R$ sufficiently large satisfying the conditions $e^{(1-\delta)R\Gamma}>1$ and $R>\frac{1}{\delta\Gamma}\log\frac{8CTn B_1}{A_1}$. This completes the proof of the theorem via contradiction.
\end{proof}

\subsection{Proof of Lemme~\ref{lem not optimal} }

\begin{proof} The key to the proof is establishing that $R\cdot\pb(\bet)\in \text{cone}(\bal)$ for large $R$. This simply follows from the fact that $\pb(\bet)$ separates its own tokens from rest i.e.
\[
\min_{i\in[n]}\max_{t\in\Tc_i}\min_{\tau\in\Tcb_i}\pb(\bet)^\top(\kb_{it}-\kb_{i\tau})\geq \min_{i\in[n]}\min_{\tau\neq\beta_i}\pb(\bet)^\top(\kb_{i\beta_i}-\kb_{i\tau})\geq 1.
\]
To proceed, suppose $\lim_{R\rightarrow \infty}\prl{R}/R\rightarrow \ps(\bal)$. Then, since tokens $\alpha_i$ will be selected (with softmax probabilities converging to $1$), $\Lc(\prl{R})\rightarrow\frac{1}{n}\sum_{i=1}^n \ell(\bgam_{i\alpha_i})$. On the other hand, since $\pb(\bet)\in \text{cone}(\bal)$ is also max-margin separating direction, we have $\lim_{R\rightarrow \infty}\Lc(R\cdot\pb(\bet))=\frac{1}{n}\sum_{i=1}^n \ell(\bgam_{i\beta_i})$. This implies $\lim_{R\rightarrow \infty}\Lc(\prl{R})>\lim_{R\rightarrow \infty}\Lc(R\cdot\pb(\bet))$ which contradicts with the optimality of $\prl{R}$ for sufficiently large $R>0$.
\end{proof}
%\textbf{Limit fails for not local-optimal.} 
