# Supplementary material for: Max-Margin Token Selection in Attention Mechanism
Source: arXiv:2306.13596 source file (2023-12-08)
Supplement: Supplementary file 3 [file app_reg_path.tex]

\section{Proofs on Regularization Path}

\subsection{Proof of Theorem \ref{meta thm}}

\begin{proof} The key idea is showing that, thanks to the exponential tail of softmax-attention, (harmful) contribution of the \irel token with the minimum margin can dominate the contribution of all other tokens as $R\rightarrow\infty$. This high-level approach is similar to earlier works on implicit bias of gradient descent with logistic loss.

Pick $\ps\in \Pc^\svm$ and set $\pb^\st_R=R\frac{\ps}{\tn{\ps}}$. This will be the baseline model that $\pb_R$ has to compete against. Also let $\pbb_R=\Gamma\frac{\pb_R}{R}$. Now suppose $\dist{\pbb_R, \Pc^\svm}\not\rightarrow0$ as $R\rightarrow\infty$. Then, there exists $\delta>0$ such that, we can always find arbitrarily large $R$ obeying $\dist{\pbb_R, \Pc^\svm}\geq \delta$.

Since $\pbb_R$ is $\delta>0$ bounded away from $\Pc^\svm$, $\pbb_R$ and $\tn{\pbb_R}=\tn{\ps}$, $\pbb_R$ strictly violates at least one of the inequality constraints in \eqref{svm}. Otherwise, we would have $\pbb_R\in \Pc^\svm$. Without losing generality, suppose $\pbb_R$ violates the constraint $m_1\geq 1$, that is, for some $\gamma:=\gamma(\delta)>0$, $\max_{t_1\in \Rc_{i}}\min_{t_0\in \Rcb_{i}}\pb^\top(\kb_{it_1}-\kb_{it_0})\leq 1-\gamma$. Now, we will argue that this will lead to a contradiction as $R\rightarrow\infty$ since we will show that $\Lc(\pb^\st_R)<\Lc(\pb_R)$ for sufficiently large $R$.

First, let us control $\Lc(\pb^\st_R)$. We study $\ab^\st_i=\sft{\Kb_i\pb^\st_R}$ and let $\alpha_i\in\Rc_i$ be the index $\alpha$ in \eqref{svm} for which $m_i\geq 1$ is attained. Then, we bound the \irel $s^\st_i$ of $\pb^\st_R$ as
\[
s^\st_i=\frac{\sum_{t\in \Rcb_{i}}\exp(\kb_{it}^\top \pb^\st_R)}{\sum_{t\in [T]}\exp(\kb_{it}^\top \pb^\st_R)}\leq \frac{\sum_{t\in \Rcb_{i}}\exp(\kb_{it}^\top \pb^\st_R)}{\exp(\kb_{i\alpha_i}^\top \pb^\st_R)}\leq T\exp(-R/\Gamma).
\]
Thus, $s^\st_{\max}=\max_{i\in [n]}s^\st_i\leq T\exp(-R/\Gamma)$. Secondly, we wish to control $\Lc(\pb_R)$ by lower bounding the irrelevance in $\pb_R$. Focusing on $m_1$, let $\alpha\in\Rc_1$ be the index in \eqref{svm} for which $m_1\leq 1-\gamma$ is attained. Denoting \irel weight-sum in the first input as $\hat{s}_1$, we find
\[
\hat{s}_1=\frac{\sum_{t\in \Rcb_{1}}\exp(\kb_{1t}^\top \pb_R)}{\sum_{t\in [T]}\exp(\kb_{1t}^\top \pb_R)}\geq \frac{1}{T}\frac{\sum_{t\in \Rcb_{1}}\exp(\kb_{1t}^\top \pb_R)}{\exp(\kb_{1\alpha}^\top \pb_R)}\geq T^{-1}\exp(-R(1-\gamma)/\Gamma).
\]
We similarly have $s^\st_{\max}\geq T^{-1}\exp(-R\Gamma)$. In conclusion, for $\pb_R,\pb^\st_R$, denoting maximum irrelevances by $\hat{s}_{\max}\geq \hat{s}_1$ and $s^\st_{\max}$, we respectively obtained 
\begin{align}\label{smax difference}
\log(\hat{s}_{\max})&\geq -(1-\gamma)(R/\Gamma)-\log T,\\
    -(R/\Gamma)-\log T\leq \log(s^\st_{\max})&\leq -(R/\Gamma)+\log T.
\end{align}
The above inequalities satisfy Assumption \ref{asshurt} as follows where $\pb\gets\pb^\star_R$ and $\pb'\gets \pb_R$: Set $R_0=3\gamma^{-1}\Gamma\log T$ so that $\log T\leq \frac{\gamma R_0}{3\Gamma}$. Secondly, set $\rho_0=-(R_0/\Gamma)-\log T$. This way, $\rho_0\geq \log(s^\st_{\max})$ implies $R\geq R_0$ and $\log T\leq \frac{\gamma R}{3\Gamma}$. To proceed, using the latter inequality, we bound the $\log T$ terms to obtain
\begin{itemize}
\item $\log(\hat{s}_{\max})\geq -(1-2\gamma/3)(R/\Gamma)$.
\item $\log(s^\st_{\max})\leq -(1-\gamma/3)(R/\Gamma)$.
\end{itemize}
To proceed, we pick $1+\Delta=\frac{1-\gamma/3}{1-2\gamma/3}$ implying $\Delta:=\frac{\gamma}{3-2\gamma}$. Finally, for this $\Delta$, there exists $\rho(\Delta)$ which we need to ensure $\log(\hat{s}_{\max})\leq \rho(\Delta)$. This can be guaranteed by picking sufficiently large $R$ that ensures $\log(s^\st_{\max})\leq -(1-\gamma/3)(R/\Gamma)\leq \rho(\Delta)$ to satisfy all conditions of Assumption \ref{asshurt}. Since such large $R$ exists by initial assumption $\dist{\pbb_R, \Pc^\svm}\not\rightarrow0$, Assumption \ref{asshurt} in turn implies that $\Lc(\pb^\st_R)<\Lc(\pb_R)$ contradicting with the optimality of $\pb_R$ in \eqref{NPT loss}.
\end{proof}

% for sufficiently small $$ $R\geq R_0$ (which exists by initial assumption)
The following example% will be further elaborated in Section \ref{sec:linear data} and 
shows that if \irel tokens result in label noise, Assumption \ref{asshurt} holds. The high-level idea behind this lemma is that, if the optimal risk is achieved by setting $\s^{\pb}_{\max}=0$, then, Assumption \ref{asshurt} will hold.%and $s_{\max}^{\pb}=\max_{i\in[n]}s^{\pb}_i$ 
\begin{lemma} [Linear label mixing] \label{label mix}Recall $s^{\pb}_i=\sum_{t\in \Rcb_t}\ab_{it}$ from Assumption \ref{asshurt}. Suppose $\link{\X_i^\top \ab_i}=\nu(1-s_i^{\pb})Y_i+Z_i$ for some $\nu> 0$. Here $Z_i=Z_i(\pb)$ is a label-noise variable induced by the \irel tokens. For some $C>0,1>\eps>0$ and for all $\pb$, we assume followings hold almost surely:
\[
|Z_i|\leq Cs^{\pb}_{\max}\quad \text{and}\quad |\E Z_i|\leq \eps\nu s_i^{\pb} |Y_i|.
\]
Consider the expected loss over $Z_i$, namely, $\bar{\Lc}(\pb):=\E_{(Z_i)_{i=1}^n}[\Lc(\pb)]$. Then, Assumption \ref{asshurt} holds for $\bar{\Lc}(\pb)$ when either of the following conditions hold:
    \begin{itemize} 
        \item Suppose $\ell(\cdot)$ is the squared loss, labels $Y_i$ are arbitrary but nonzero, and $\nu\leq 1$.
        \item Suppose $\ell(\cdot)$ is the logistic loss, labels $Y_i\in\{-1,1\}$, and $\nu>0$ is arbitrary.
    \end{itemize}
\end{lemma}

\subsection{Application to Linearly-mixed Labels}
\begin{lemma} [Linear label mixing] \label{label mix}Recall $s^{\pb}_i=\sum_{t\in \Rcb_t}\abp_{it}$ from Assumption \ref{asshurt}. Suppose $\link{\X_i^\top \abp_i}=\nu_i(1-s_i^{\pb})Y_i+Z_i$ for some $(\nu_i)_{i=1}^n>0$ and all $i\in[n]$. Here $Z_i=Z_i(\pb)$'s correspond to ``label-corruption'' variables induced by the \irel tokens. Importantly, we will allow $Z_i$'s to be stochastic. For some $C>0,1>\eps>0$ and for all $\pb\in\R^d$, we assume the followings hold almost surely:
    \[
    |Z_i|\leq Cs^{\pb}_{\max}\quad \text{and}\quad |\E Z_i|\leq \eps\nu_i s_i^{\pb} |Y_i|.
    \]
    Consider the expected loss\footnote{In the simpler setting of Section \ref{}, $Z_i$ is deterministic and the result applies by setting $Z_i=\E[Z_i]$.} over $Z_i$, namely, $\bar{\Lc}(\pb):=\E_{(Z_i)_{i=1}^n}[\Lc(\pb)]$. Then, Assumption \ref{asshurt} holds for $\bar{\Lc}(\pb)$ when either of the following conditions hold:
        \begin{itemize} 
            \item Suppose $\ell(\cdot)$ is the squared loss, labels $Y_i$ are arbitrary but nonzero, and $\nu\leq 1$.
            \item Suppose $\ell(\cdot)$ is the logistic loss, labels $Y_i\in\{-1,1\}$, and $\nu>0$ is arbitrary.
        \end{itemize}
    \end{lemma}
    \begin{proof} \noindent\textbf{$\bullet$ Case 1: Squared loss.} Let us first consider the squared loss $(Y_i-\hat{Y}_i)^2$. Let $M_+=\max_{i\in[n]}Y_i^2,M_-=\min_{i\in[n]}Y_i^2>0$. Define $\Lc'(\pb):=\bar{\Lc}(\pb)-\frac{1}{n}\sum_{i=1}^n(1-\nu)^2Y_i^2$ where $\frac{1}{n}\sum_{i=1}^n(1-\nu)^2Y_i^2$ is the minimum achievable risk by setting $s_{\max}=0$ whenever $\nu\leq 1$. Set $\mu_i:=\E[Z_i]/(\nu s_i^{\pb}Y_i)$ and recall $|\mu_i|\leq \eps$. Set $\kapp:=\nu s_{\max}$. We have that
    %$\sigma_{\max}^2=\max_{i\in[n]}\sigma_i^2$%Denote $\E[Z_i^2]\leq C^2s_{\max}^2$
        \begin{align}
        \Lc'(\pb)&=\frac{1}{n}\sum_{i=1}^n\E_{Z_i}[(Y_i-\nu (1-s_i)Y_i-Z_i)^2]-\frac{1}{n}\sum_{i=1}^n(1-\nu)^2Y_i^2\\
        &= \frac{1}{n}\sum_{i=1}^n((1-\nu+\nu s_i(1-\mu_i))^2-(1-\nu)^2)Y_i^2+\text{var}[Z_i]\\
        &=\frac{1}{n}\sum_{i=1}^n\nu s_i(1-\mu_i)(2-2\nu+\nu s_i(1-\mu_i))Y_i^2+\text{var}[Z_i]\\
        &\geq B:=(1-\eps)^2\kapp(2-2\nu+\kapp)M_-/n.
        %&\geq (1-\eps)^2\kappa^2M_-/n.
        \end{align}
        Using the identical argument and the upper bound $\E[Z_i^2]\leq C^2s_{\max}^2$, we also obtain an upper bound
        \[
        \Lc'(\pb)\leq (1+\eps)^2\kapp(2-2\nu+\kapp)M_++C^2s_{\max}^2.
        \]
        %$s_{\max}\leq 1$ and 
        Now, independent of the choice of $\pb$, the ratio of upper/lower bounds obey (using $\kapp(2-2\nu+\kapp)\geq \nu s_{\max}^2$)
        \[
        \frac{(1+\eps)^2\kapp(2-2\nu+\kapp)M_++C^2s_{\max}^2}{B}\leq n\frac{(1+\eps)^2M_++C^2/\nu}{(1-\eps)^2M_-}:=\Theta.
        \] 
        %Recalling $s_{\max}:=\max_{i\in[n]}s_i$, clearly,
        %Setting $B:=(1-\nu+\nu s_{\max})\sqrt{M_-/n}$, 
        Overall, we found $\sqrt{\Theta}B\geq \sqrt{\Lc'(\pb)}\geq B$. Thus, for any $\pb,\pb'$, we have that, if $\sqrt{\Theta } s^{\pb}_{\max}(2-2\nu+\nu s^{\pb}_{\max})< s^{\pb'}_{\max}(2-2\nu+\nu s^{\pb'}_{\max})$, then $\Lcb(\pb)< \Lcb(\pb')$. Note that the former condition is implied by the stricter but cleaner criteria $\sqrt{\Theta } s_{\max}^{\pb}< s_{\max}^{\pb'}$.
        
        Going back to the condition of Assumption \ref{asshurt}, any $\log (s^{\pb}_{\max})\leq (1+\Delta)\log (s^{\pb'}_{\max})$ obeys $s^{\pb}_{\max}\leq (s^{\pb'}_{\max})^{1+\Delta}$ i.e. $s^{\pb'}_{\max}\geq (s^{\pb}_{\max})^{(1+\Delta)^{-1}}$. Following above, we wish to ensure $s^{\pb'}_{\max}>\sqrt{\Theta}s^{\pb}_{\max}$ for such $(\pb,\pb')$ pairs. This is guaranteed by
        \[
        (s^{\pb}_{\max})^{(1+\Delta)^{-1}-1}>\sqrt{\Theta}\iff \frac{\Delta}{1+\Delta}\log(s^{\pb}_{\max})< -0.5\log(\Theta).
        \]
        The above is satisfied by choosing a $\rho(\Delta):=-(1+\Delta^{-1})\log(\Theta)$ in Assumption \ref{asshurt}.
    
        \noindent\textbf{$\bullet$ Case 2: Logistic loss.} Logistic loss is \rel because (i) it is used in most classification problems and also (ii) softmax-attention and logistic loss are both exponential-tailed so their joint interaction is of practical interest for transformers. To proceed, let us write the logistic loss in a similar fashion where we use $\ell(Y,\hat{Y})=\ell(Y\hat{Y})=\log(1+e^{-Y\hat{Y}})$. Let $Z'_i=Y_iZ_i$ which is zero-mean with same variance. 
        \begin{align*}
            \bar{\Lc}(\pb)&=\frac{1}{n}\sum_{i=1}^n\E_{Z_i}[\ell(Y_i(\nu(1-s_i^{\pb})Y_i+Z_i))]\\
            &=\frac{1}{n}\sum_{i=1}^n\E_{Z_i}[\ell(\nu(1-s_i^{\pb})+Z'_i)].
            %&=\frac{-1}{2n}\sum_{i=1}^n[\log((1-s_i^{\pb})+s_i^{\pb} \eps)+\log((1-s_i^{\pb})-s_i^{\pb} \eps)]\\
            %&=\frac{-1}{2n}\sum_{i=1}^n\log((1-s_i^{\pb})^2-\eps^2s_i^{\pb})
            \end{align*}
        Compared to squared loss, here we describe a more general approach that leverage Lipschitzness under small perturbations. Pick a sufficiently small $\rho_0:=\rho_0(\nu)$ and assume $s_{\max}^{\pb}\leq \rho_0$. Then, for $|\gamma|\leq s_{\max}^{\pb}\leq \rho_0$, through Taylor series, we can write
        \[
        0\leq \ell(\nu+\gamma)-\ell(\nu)-\gamma\ell'(\nu)\leq \gamma^2\ell''(\nu).
        \]
        This implies the following upper/lower bounds on summands of $\bar{\Lc}(\pb)$: Setting $\mu_i=\E[Z'_i]/(\nu s_i^{\pb})$, using $|\mu_i|\leq \eps$, $|Z_i|\leq Cs_{\max}^\pb$, and convexity of $\ell(\nu)$
        \[
        0\leq \E_{Z_i}[\ell(\nu(1-s_i^{\pb})+Z'_i)]-\ell(\nu)+(1-\mu_i)\nu s_i^{\pb}\ell'(\nu)\leq (\nu+C)^2s_{\max}^2.
        \]
        Set $\Lc'(\pb):=\Lc(\pb)-\ell(\nu)$ where $\ell(\nu)$ is the minimum achievable loss (thanks to the convexity of $\ell$). Since $\ell$ is strictly decreasing, $\Theta:=-\ell'(\nu)>0$. To proceed, we obtain
        \[
        (\nu+C)^2s_{\max}^2+\Theta(1+\eps)\nu s_{\max}\geq \Lc'(\pb)\geq n^{-1}\Theta(1-\eps)\nu s_{\max}.
        \]
        We now repeat the similar argument as squared loss: For any $\pb,\pb'$, we have that, if $(\nu+C)^2(s^{\pb}_{\max})^2+\Theta(1+\eps)\nu s^{\pb}_{\max}< n^{-1}\Theta(1-\eps)\nu s^{\pb'}_{\max}$, then $\Lcb(\pb)< \Lcb(\pb')$. Note that this condition is implied by the stricter but cleaner criteria $\bar{\Theta}s^{\pb}_{\max} < s^{\pb'}_{\max}$ with $\bar{\Theta}:=n(1-\eps)^{-1}(\Theta^{-1}\nu^{-1}(\nu+C)^2\rho_0+1+\eps)$ thanks to $s^{\pb}_{\max}\leq \rho_0$. Note that $\bar{\Theta}$ is independent of $\pb$ for any $s_{\max}^{\pb}\leq \rho_0$.
    
        Going back to the condition of Assumption \ref{asshurt}, any $\log (s^{\pb}_{\max})\leq (1+\Delta)\log (s^{\pb'}_{\max})$ obeys $s^{\pb}_{\max}\leq (s^{\pb'}_{\max})^{1+\Delta}$ i.e. $s^{\pb'}_{\max}\geq (s^{\pb}_{\max})^{(1+\Delta)^{-1}}$. Following above, we wish to ensure $s^{\pb'}_{\max}>\bar{\Theta}s^{\pb}_{\max}$ for such $(\pb,\pb')$ pairs. This is guaranteed by
        \[
        (s^{\pb}_{\max})^{(1+\Delta)^{-1}-1}>\bar{\Theta}\iff \frac{\Delta}{1+\Delta}\log(s^{\pb}_{\max})< -\log(\bar{\Theta}).
        \]
        The above is satisfied by choosing a $\rho(\Delta):=-2(1+\Delta^{-1})\log(\bar{\Theta})$ in Assumption \ref{asshurt}. Thus, setting $\rho=\min(\rho(\Delta),\log \rho_0)$, any $\log (s^{\pb}_{\max})\leq \rho$ satisfies the condition of Assumption \ref{asshurt} finishing the proof.
    \end{proof}
