# Supplementary material for: Max-Margin Token Selection in Attention Mechanism
Source: arXiv:2306.13596 source file (2023-12-08)
Supplement: Supplementary file 4 [file app_tight_local.tex]

\subsection{Proof of Theorem~\ref{local path fail main}: Regularization Path Fails for Non-Locally-Optimal Tokens}%to Converge 

The theorem below is essentially a restatement of Theorem \ref{local path fail main} and shows that regularization path does not converge to the max-margin solution if token indices $\bal$ does not satisfy Definition \ref{def loc opt}. {The only difference is that, Theorem \ref{local path fail main} replaces the second condition below with a cleaner statement which assumes the linear-independence of the support vectors.}
\begin{theorem} [Failure of Local Regularization Path]\label{local path fail} Fix token indices $\bal=(\alpha_i)_{i=1}^n$ with \neis $(\Tc_i)_{i=1}^n$. Suppose for some $j\in[n]$, there exists an \nei $\beta\in\Tc_j$ satisfying the following:
\begin{itemize}
\item $\x_{j\beta}$ has a higher score than $\x_{j\alpha_j}$: $Y_j\cdot\vb^\top \x_{j\beta}>Y_j\cdot\vb^\top \x_{j\alpha_j}$.
\item Recall $\ps=\ps(\bal)$ be the solution of \eqref{attnsvm} and let $\psp$ be the solution of \eqref{attnsvm} where the constraint $(\kb_{j\alpha_j}-\kb_{j\beta})^\top\pb\geq 1$ is not enforced. $\beta$ is an \emph{active} \nei in the sense that $\psp$ violates the constraint i.e.~$(\kb_{j\alpha_j}-\kb_{j\beta})^\top\psp< 1$.

%$\beta$ is an \emph{efficient} \nei in the sense that $\psp$ achieves strictly smaller margin on that constraint i.e.~$(\kb_{i\alpha_i}-\kb_{i\beta})^\top(\psp/\tn{\psp}-\ps/\tn{\ps})$.

%consider the SVM without the constraint at $\beta$ i.e. $\ps^\top(\kb_{i\alpha_i}-\kb_{i\beta})=1$ is efficient in the sense that, 
%Set $\bet\in\R^n$ with $\beta_i=\alpha_i$ for all $i\neq j$ and $\bet_j=\beta$. Consider \eqref{attnsvm} solution $\pb(\bet)$. 
\end{itemize}
For any $\eps>0$, there exists $R_\eps>0$ as follows: Consider the neighborhood of $\ps$: $\Cc_{\eps}=\cone_{\eps}(\ps)$ $\bigcap\left\{\pb~|~\tn{\pb}\geq R_\eps\right\}$. Define the local path $\pbb(R)=\min_{\pb\in \Cc_{\eps},\tn{\pb}\leq R}\Lc(\pb)$. Then $\underset{R\rightarrow\infty}{\lim}\frac{\pbb(R)}{\tn{\pbb(R)}}\neq \frac{\ps}{\tn{\ps}}$.
\end{theorem}

\textbf{Proof of Theorem \ref{local path fail main}:} Using the above theorem we can now conclude the proof of Theorem \ref{local path fail main} by showing that, second bullet of Theorem \ref{local path fail main} implies the second bullet of Theorem \ref{local path fail}. We are given solution $\ps$ and $\pb^\beta$. Suppose that $\pb^\beta$ in Theorem \ref{local path fail main} does not violate the constraint $(\kb_{j\alpha_j}-\kb_{j\beta})^\top\psp\geq 1$. Then, it would imply that $\pb^\beta=\ps$ because $\pb^\beta$ satisfies all margin constraints and $\tn{\pb^\beta}\leq \tn{\ps}$ (because it solves the problem with less constraints), thus, if $\pb^\beta\neq \ps$, it would contradict with the optimality of $\ps$. Since the active constraints are linearly independent, their Lagrange multipliers are unique. Since $\pb^\beta$ is missing a linearly independent constraint, the solution $\pb^\beta$ expressed in terms of Lagrange-weighted constraints cannot equate to the solution $\ps$ expressed in terms of its own Lagrange-weighted constraints that also include the constraint induced by $\kb_{j\alpha_j}-\kb_{j\beta}$.
%let us consider their active constraints and observe that $\pb^\beta$ (when solving the problem without $\beta$-constraint) has one less active constraint than $\ps$. 

%Step 1: We have solution $\ps$. Remove constraint 1 and suppose it still gets satisfied. The solution has to be same because old constrains still hold. Since solution is same, active set is same. But the second active set is missing an element. But KKT solution is unique hence contradiction

%Let's assume that $\psp$ does not violate the constraint, i.e., $ (\kb_{j\alpha_j}-\kb_{j\beta})^\top\psp = 1 $. Consequently, the problem \eqref{attnsvm} with and without the additional active constraint $(\kb_{j\alpha_j}-\kb_{j\beta})^\top\pb = 1$ will have the same solution. On the other hand, since the objective in \eqref{attnsvm} is strongly convex, and the constraints are linearly independent based on our assumption, the Mangasarian-Fromovitz constraint qualification guarantees a unique KKT solution \cite{mangasarian1994nonlinear}. However, this leads to a contradiction.

\subsubsection{Proof of Theorem~\ref{local path fail}}

%\begin{proof} 
\noindent\textbf{Proof strategy:} Without losing generality, let us prove the result for $2\eps$ (to simplify the downstream notation). To accomplish the proof, we will follow the following strategy. Fix $\pseb=\frac{\eps\psp+(1-\eps)\ps}{\tn{\eps\psp+(1-\eps)\ps}}$ and $\psb=\ps/\tn{\ps}$. Using $\tn{\pb^\beta}\leq \tn{\ps}$, we observe that $\pseb$ obeys the correlation inequality
\[
(\pseb)^\top \psb\geq \frac{(1-\eps)\tn{\ps}^2-\eps\tn{\ps}\tn{\psp} }{\tn{\ps}((1-\eps)\tn{\ps}+\eps\tn{\psp})}\geq \frac{(1-2\eps)\tn{\ps}^2}{\tn{\ps}^2}\geq 1-2\eps.
\]
This establishes that $r\cdot\pseb\in \cone_{2\eps}(\ps)$. Thus, we will use $\pseb$ to show that it is a superior direction to $\ps$. Concretely, for all $R\geq R_\eps$, suppose that, there exists $\delta=\delta(\eps)$ such that, 
\begin{align}
\Lc(R\cdot\pseb)<\inf_{\tn{\pb}=R,\pb\in \cone_{\delta}(\ps)}\Lc(\pb).\label{delta is worse}
\end{align}
In words, suppose that $R\cdot\pseb$ achieves strictly better loss than all points of $\ell_2$-norm $R$ within $\cone_{\delta}(\ps)$. Establishing this would imply the desired result $\underset{R\rightarrow\infty}{\lim}\frac{\pbb(R)}{\tn{\pbb(R)}}\neq \frac{\ps}{\tn{\ps}}$. Since for any choice of $R\geq R_\eps$, \eqref{delta is worse} implies that the optimal direction $\frac{\pbb(R)}{\tn{\pbb(R)}}$ is at least $\delta$ bounded away from $\frac{\ps}{\tn{\ps}}$. In what follows, we will prove this by establishing \eqref{delta is worse}.

First, let us establish the critical properties of $\psp$. Set $K=n(T-1)$ and gather the set of margin equalities $\ps:=\ps(\bal)$ satisfies: These inequalities are given by vectors $(\vb_{k=1}^K)$ where $\vb_k$ is the form $\kb_{\alpha_i}-\kb_{t}$ for $t\neq\alpha_i$. Also let $\vb_1=\kb_{j\alpha_j}-\kb_{j\beta}$ be the active constraint described in the theorem.

Note that $\tn{\psp}\leq \tn{\ps}$ since $\psp$ is solving a max-margin problem with strictly less constraints (over $k\geq 2$). Secondly, we claim that $\psp$ achieves a strictly larger margin compared to $\ps$ over $k\geq 2$, namely setting $\Gamma=\tn{\ps}$ and $\Gamma_\beta=\tn{\psp}$
\begin{align}
\min_{k\geq 2}\vb_k^\top\psp/\tn{\psp}=1/\Gamma_\beta>\min_{k\geq 2}\vb_k^\top\ps/\tn{\ps}=1/\Gamma.\nonumber
\end{align}
If not, it would imply that $\tn{\psp}=\tn{\ps}$ and that $\min_{k\geq 2}\vb_k^\top\ps=\min_{k\geq 2}\vb_k^\top\psp$. Since theorem's statement guarantees $\ps\neq\psp$, this contradicts with the unique optimality of $\psp$ when satisfying constraints $k\geq 2$ as $\ps$ would achieve the same objective.%Otherwise, it would contradict with the optimality of $\psp$ over  since 

Finally, using same argument, we also note that, $\psp$ achieves strictly less margin over $\vb_1$, namely
\begin{align}
\vb_1^\top\psp/\tn{\psp}<\vb_1^\top\ps/\tn{\ps}=1/\Gamma.\label{useful eq first}
\end{align}
If not, it would imply that $\psp$ achieves a better or equal margin at all constraints which would contradict with the optimality of $\ps$ over constraints $k\geq 1$.

Now, let us define $\pse=\eps\psp+(1-\eps)\ps$ and observe that $\pse$ also satisfies the discussion above. Namely, using $\tn{\pse}\leq \eps\tn{\psp}+(1-\eps)\tn{\ps}<\Gamma$ we find
\begin{align}
\frac{\min_{k\geq 2}\vb_k^\top\pse}{\tn{\pse}}\geq \frac{1}{\eps\tn{\psp}+(1-\eps)\tn{\ps}}>\frac{1}{\Gamma}.\label{gamt eq}%=\frac{1}{\gamt}
\end{align}
Similarly, on constraint $\vb_1$, we have that
\begin{align}
\vb_1^\top\pse/\tn{\pse}:=1/\gamp<1/\Gamma.\label{useful eq}
\end{align}
If not, it would imply that $\pse$ achieves a better or equal margin on all constraints which would contradict with the unique optimality of $\ps$ over constraints $k\geq 1$.

We will use $\gamp>\Gamma$, \eqref{useful eq}, and \eqref{gamt eq} to conclude that $\pse$ is a strictly better direction compared to a $\delta=\delta(\eps)$ conic neighborhood of $\psb:=\ps/\tn{\ps}$. Pick the $\delta$ neighborhood of $\ps$ such that, all $\psd$ it satisfies
\begin{align}
&\vb_k^\top\psd/\tn{\psd}\geq 1/\damp=0.5(1/\gamp+1/\Gamma)>1/\gamp\quad\text{for all}\quad k\in[K].\label{damp eq}
%&\vb_1^\top\psd/\tn{\psd}\geq1/\damp=0.5(1/\gamp+1/\Gamma)>1/\gamp.
\end{align}
In words, we choose a neighborhood with correlation profile dominated by $\pse$ (on $k=1$ and $k\geq 2$). We now lower bound the loss function over $\delta$-neighborhood and upper bound over $\pse$. Specifically, we will compare a $\psd$ within the $\delta$ neighborhood of $\ps$ with $\tn{\psd}=R$ and $\pset:=R\cdot\pseb$. To proceed, define:
\[
q^\st_i=1-\sft{\Kb_i\pset}_{\alpha_i},\quad \hat{q}_i=1-\sft{\Kb_i\psd}_{\alpha_i}
\]
Also define $q^\beta=\sft{\Kb_j\pset}_{\beta}$ which is the $j$'th softmax likelihood at token $\beta$. We will use the fact that margin at $\beta$ is small for $j$'th example to lower bound $q^\beta$ carefully. We next bound these as follows based on \eqref{useful eq}, \eqref{gamt eq}, \eqref{damp eq} (e.g.~following derivation of \eqref{smax difference})\footnote{We are essentially following identical arguments developed in the proofs of Theorem \ref{meta thm} or Theorem \ref{thm:path:joint:vp}.}
\begin{equation}\label{q bounds fail}
\begin{split}
&\log(q^\st_i)\leq -(R/\Gamma)+\log T\quad\text{for all}\quad i\neq j\\
&\log(q^\beta)\geq -(R/\gamp)-\log T\quad\text{for all}\quad i\neq j\\
&\log(q^\st_j-q^\beta)\leq -(R/\Gamma)+\log T\quad\text{for all}\quad i\neq j\\
&\log(\hat{q}_i)\leq -(R/\damp)+\log T\quad\text{for all}\quad i\in[n].
\end{split}
\end{equation}
$\bullet$ \textbf{Lower bounding $\Lc(\psd)$:} Using the last inequality, on $\psd$ (within the $\delta$ neighborhood of $\ps$), we have the following lower bound: Set $\x^\delta_i=\X_i^\top\sft{\Kb_i\psd}$ and $M:=\sup_{i\in[n],t,\tau\in[T]}\tn{\x_{it}-\x_{i\tau}}$ and note that $\tn{\x^\delta_i-\x_{\alpha_i}}\leq M\hat{q}_i$. Also let $B$ and $A$ be the lower and upper bound of $-\ell'$ over $[-M\tn{\vb},M\tn{\vb}]$ interval. Finally, define $\Lc_\st=\frac{1}{n}\sum_{i=1}^n \ell(\vb^\top\x_{i\alpha_i})$. We find
\begin{equation}\label{psd bound}
\begin{split}
|\Lc(\psd)-\Lc_\st|&=\frac{1}{n}\sum_{i=1}^n|\ell(Y_i\cdot\vb^\top \x^\delta_i)-\ell(Y_i\cdot\vb^\top \x_{i\alpha_i})|\\
&\leq B\hat{q}_{\max} M\tn{\vb}\\
&\leq TBM\tn{\vb} e^{-R/\damp}.
\end{split}
\end{equation}

This implies $\Lc(\psd)\geq \Lc_\st-TBM\tn{\vb} e^{-R/\damp}$. Note that this holds for all $\psd$ within the conic neighborhood $\cone_{\delta}(\ps)\cap \{\pb\bgl\tn{\pb}=R\}$ (defined above \eqref{delta is worse}).

$\bullet$ \textbf{Upper bounding $\Lc(\pset)$:} On $\pse$, we upper bound the loss as follows. Define the loss $\Lc^{-j}(\pb)=\frac{1}{n}\sum_{i\neq j}\ell(Y_i\cdot f(\X_i))$ i.e.~loss over all training data except the $j$'th one. Repeating the argument identical to \eqref{psd bound}, we find that
\[
|\Lc^{-j}(\pset)-\Lc^{-j}_\st|\leq TBM\tn{\vb} e^{-R/\Gamma}.
\]
The critical term is the $j$'th loss which we need to upper bound as follows. Set $\x^\eps_j=\X_j^\top \sft{\Kb_j\pset}$ and define the score improvement by $\beta$ to be $\bgag=Y_j\cdot\vb^\top(\x_{i\beta}-\x_{j\alpha_j})>0$. We note that
\begin{align*}
Y_j\cdot\vb^\top\x^\eps_j-Y_j\cdot\vb^\top \x_{\alpha_j}&=q^\beta Y_j\cdot\vb^\top(\x_{i\beta}-\x_{\alpha_j})+\sum_{t\notin\{\alpha_j,\beta\}}  \sft{\Kb_j\pset}_{t}Y_j\cdot\vb^\top(\x_{it}-\x_{\alpha_j})\\
&\geq q^\beta\bgag-(q^\st_j-q^\beta)M\tn{\vb}\\
&\geq T^{-1}\bgag e^{-R/\gamp}-TBM\tn{\vb} e^{-R/\Gamma}.
\end{align*}
Combining these into $\Lc(\pset)=\Lc^{-j}(\pset)+n^{-1}\ell(Y_j\cdot\vb^\top\x^\eps_j)$ and using $A\leq -\ell'\leq B$, we obtain the lower bound
\begin{align*}
\Lc(\pset)-\Lc_\st\leq 2TBM\tn{\vb} e^{-R/\Gamma}-An^{-1}T^{-1}\bgag e^{-R/\gamp}.
\end{align*}
In conclusion, we find that $\Lc(\pset)>\Lc(\psd)$ whenever
\[
An^{-1}T^{-1}\bgag e^{-R/\gamp}>2TBM\tn{\vb} (e^{-R/\Gamma}+ e^{-R/\damp}).
\]
Using the relationship $\gamp\geq \damp\geq \Gamma$ and noticing $1/\damp-1/\gamp=(1/\Gamma-1/\gamp)/2$, this is implied by
\[
e^{R(1/\damp-1/\gamp)}>4T^2nBMA^{-1}\tn{\vb}\iff R>\frac{2\gamp \Gamma}{\gamp-\Gamma}\log(4T^2nBMA^{-1}\tn{\vb}).
\]
Thus, as advertised, we found that, for any $\eps>0$, there exists $R_\eps$ such that, over the set $\cone_{\eps}(\ps)\bigcap\{\pb\bgl \tn{\pb}\geq R_\eps\}$, $\pset$ with $\tn{\pset}=R>R_\eps$ achieves smaller loss compared to $\Lc(\psd)$ for all $\psd\in \cone_{\delta}(\ps)\bigcap\{\pb\bgl \tn{\pb}=R\}$. This in turn implies \eqref{delta is worse} for all $R>R_\eps$ concluding the proof.
%that $\pbb(R)/R\not\rightarrow \ps$ since $\pbb(R)$ lies outside of $\cone_{\delta}(\ps)$ (a small conic/directional neighborhood around $\ps$).
%\end{proof}
