# Supplementary material for: Max-Margin Token Selection in Attention Mechanism
Source: arXiv:2306.13596 source file (2023-12-08)
Supplement: Supplementary file 6 [file bc_app_local.tex]

\section{Analysis of the Local Regularization Path}

\begin{definition}[SVM-neighbor and locally-optimal tokens]\label{def loc opt} Fix token indices $\bal=(\alpha_i)_{i=1}^n$. Solve \eqref{attnsvm} to obtain $\ps=\ps(\bal)$. Consider tokens $\Tc_i\subset[T]$ such that $(\kb_{i\alpha_i}-\kb_{it})^\top \ps=1$ for all $t\in\Tc_i$. We refer to $\Tc_i$ as SVM-neighbor of $\kb_{i\alpha_i}$. Additionally, tokens $\bal=(\alpha_i)_{i=1}^n$ are called locally-optimal if for all $i\in[n]$, $t\in\Tc_i$, we have that $\vb^\top (\x_{i\alpha_i}-\x_{it})>0$. 
    % For each $i\in[n]$, define the set of SVM-neighbors of $\alpha_i$ to be
    \end{definition}
    
    \begin{assumption} [Regularity condition for GD]\label{ass regular} Fix token indices $\bal=(\alpha_i)_{i=1}^n$ and let $\Tc_i\subset[T]$ be their SVM-neighbors for $i\in[n]$. Either of the following holds:
    \begin{enumerate}
    \item \textbf{Same scores:} For all $i\in[n]$ and $t_1,t_2\in\Tc_i$, $\kb_{it_1}^\top\ps=\kb_{it_1}^\top \ps$.
    \item \textbf{Low-score SVM-neighbor is separable:} Set $\tau_i=\arg\min_{t\in \Tc_i}\vb^\top \x_t$. There exists $\qb\in\R^d$ such that $\min_{\tau\in \Tc_i-\{\tau_i\}}\qb^\top (\kb_{i\tau_i}-\kb_{it})\geq 1$ for all $i\in [n]$.
    \end{enumerate}
    \end{assumption}
    \begin{lemma}[Local Gradient Condition] Let $\bal=(\alpha_i)_{i=1}^n$ be locally-optimal tokens per Definition \ref{def loc opt} and Assumption \ref{ass regular} holds. Define the set $\text{cone}_{\nu,R}(\ps)$ to be vectors obeying $\corr{\pb,\ps}\geq 1-\nu$ and $\tn{\pb}\geq R$. There exists $\nu>0$ such that all $\pb\in \text{cone}_{\nu,R_{\nu,\pi}}(\ps)$ with  obeys
    \[
    \li\nabla\Lc(\pb),\pbb\ri\geq (1+\pi)\li\nabla\Lc(\pb),\ps\ri.
    \]
    As a result, choosing $\pi\leq \nu/2$, gradient iterations starting within $\text{cone}_{\nu,R_{\nu,\pi}}(\ps)$ eventually obeys $\pb\in \text{cone}_{\nu/2,R_{\nu,\pi}}(\ps)$.
    \end{lemma}
    \begin{proof} Let $\ps=\ps(\bal)$ be the solution of \eqref{attnsvm}. Recall the definition $\Cc_\nu=\{\pb\in\R^d~\big|~\corr{\pb,\ps}\geq 1-\nu\}$. Let $(\Tc_i)_{i=1}^n$ be the set of all SVM-neighbors per Definition \ref{def loc opt}. Fix $\nu>0$ such that, for some $\delta>0$, for all $i\in[n], t_1\in\Tc_i,t_2\not\in\Tc_i$, we have that
    \[
    (\kb_{it_1}-\kb_{it_2})^\top \pb>\delta>0\quad\text{for all}\quad \pb\in \Cc_\nu.
    \]
    Note that such a $(\nu,\delta)$ is guaranteed to exist because SVM-neighbors achieve strictly higher correlations to $\ps$ than non-neighbors.
    
    Now that the choice of $\nu$ is determined, we need to prove the main claim. Fix $\pi>0$ and $R=R_\pi$ is to be determined. We first show that, for sufficiently large $R$, there exists a vector $\pt$ that is arbitrarily close to $\ps$ and achieves near-optimal risk. We will prove the result for Assumption \ref{ass regular}, Case 2. The proof of Case 1 follows same argument but we can simply set $\pt=\ps$.% (rather than the additional argument). % which simplifies the argument
    
    Recall definitions of $\qb$ and $(\tau_i)_{i=1}^n$ from Assumption \ref{ass regular} and set $\pt=\ps+\eps \qb$ for sufficiently small $\eps>0$ that will be chosen according to $\pi$. This choice ensures that $\tau_i$ is the second highest scoring token besides $\alpha_i$, that is, $\kb_{\tau_i}^\top \pt=\max_{t\neq \alpha_i} \kb_{it}^\top \pt$. Consequently, for sufficiently large $R=R(\eps)$, we obtain
    \[
    \]
    \end{proof}
