# Supplementary material for: Max-Margin Token Selection in Attention Mechanism
Source: arXiv:2306.13596 source file (2023-12-08)
Supplement: Supplementary file 7 [file app_local_path_iff.tex]

\section{Regularization Path Fails to Converge for Non-Locally-Optimal Tokens}% via Regularization Path

\begin{comment}
\begin{definition}[\nei and locally-optimal tokens]\label{def loc opt2} Fix token indices $\bal=(\alpha_i)_{i=1}^n$. Solve \eqref{attnsvm} to obtain $\ps=\ps(\bal)$. Consider tokens $\Tc_i\subset[T]$ such that $(\kb_{i\alpha_i}-\kb_{it})^\top \ps=1$ for all $t\in\Tc_i$. We refer to $\Tc_i$ as \neis of $\kb_{i\alpha_i}$. Additionally, tokens $\bal=(\alpha_i)_{i=1}^n$ are called locally-optimal if for all $i\in[n]$, $t\in\Tc_i$, we have that $\vb^\top (\x_{i\alpha_i}-\x_{it})>0$. 
\end{definition}
\end{comment}
The theorem below is essentially a restatement of Theorem \ref{local path fail main}. \red{The only difference is that, Theorem \ref{local path fail main} replaces the second condition below with a cleaner statement which assumes the linear-independence of the support vectors.}
\begin{theorem} [Failure of Local Regularization Path]\label{local path fail} Fix token indices $\bal=(\alpha_i)_{i=1}^n$ with \neis $(\Tc_i)_{i=1}^n$. Suppose for some $j\in[n]$, there exists an \nei $\beta\in\Tc_j$ satisfying the following:
\begin{itemize}
\item $\x_{j\beta}$ has a higher score than $\x_{j\alpha_j}$: $Y_j\cdot\vb^\top \x_{j\beta}>Y_j\cdot\vb^\top \x_{j\alpha_j}$.
\item Recall $\ps=\ps(\bal)$ be the solution of \eqref{attnsvm} and let $\psp$ be the solution of \eqref{attnsvm} where the constraint $(\kb_{j\alpha_j}-\kb_{j\beta})^\top\pb\geq 1$ is not enforced. $\beta$ is an \emph{active} \nei in the sense that $\psp$ violates the constraint i.e.~$(\kb_{j\alpha_j}-\kb_{j\beta})^\top\psp< 1$.

%$\beta$ is an \emph{efficient} \nei in the sense that $\psp$ achieves strictly smaller margin on that constraint i.e.~$(\kb_{i\alpha_i}-\kb_{i\beta})^\top(\psp/\tn{\psp}-\ps/\tn{\ps})$.

%consider the SVM without the constraint at $\beta$ i.e. $\ps^\top(\kb_{i\alpha_i}-\kb_{i\beta})=1$ is efficient in the sense that, 
%Set $\bet\in\R^n$ with $\beta_i=\alpha_i$ for all $i\neq j$ and $\bet_j=\beta$. Consider \eqref{attnsvm} solution $\pb(\bet)$. 
\end{itemize}
For any $\eps>0$, there exists $R_\eps>0$ as follows: Consider the neighborhood of $\ps$: $\Cc_{\eps}=\cone_{\eps}(\ps)$ $\bigcap\left\{\pb~|~\tn{\pb}\geq R_\eps\right\}$. Define the local path $\pbb(R)=\min_{\pb\in \Cc_{\eps},\tn{\pb}\leq R}\Lc(\pb)$. Then $\underset{R\rightarrow\infty}{\lim}\frac{\pbb(R)}{\tn{\pbb(R)}}\neq \frac{\ps}{\tn{\ps}}$.
\end{theorem}

\subsection{Proof of Theorem~\ref{local path fail}}

\begin{proof} 
Fix $\pseb=\frac{\eps\psp+(1-\eps)\ps}{\tn{\eps\psp+(1-\eps)\ps}}$. There exists $R_\eps$ such that for all $R\geq R_\eps$, $\Lc(R\cdot\pseb)<\Lc(R\cdot\psb)$ where $\psb=\ps/\tn{\ps}$.
\noindent \textbf{Remark.} In words, this theorem shows that, within arbitrarily small neighborhood around $\ps$, there is a strictly superior ray $R\cdot\pseb$. Thus, $\ps$ direction is not locally optimal (unlike Theorem \ref{thm:local:gd}). This establishes the tightness of locally-optimal token Definition \ref{def loc opt}.

First, let us establish the critical properties of $\psp$. Set $K=n(T-1)$ and gather the set of margin equalities $\ps:=\ps(\bal)$ satisfies: These inequalities are given by vectors $(\vb_{k=1}^K)$ where $\vb_k$ is the form $\kb_{\alpha_i}-\kb_{t}$ for $t\neq\alpha_i$. Also let $\vb_1=\kb_{j\alpha_j}-\kb_{j\beta}$ be the active constraint described in the theorem.

Note that $\tn{\psp}\leq \tn{\ps}$ since $\psp$ is solving a max-margin problem with strictly less constraints (over $k\geq 2$). Secondly, we claim that $\psp$ achieves a strictly larger margin compared to $\ps$ over $k\geq 2$, namely setting $\Gamma=\tn{\ps}$ and $\Gamma_\beta=\tn{\psp}$
\begin{align}
\min_{k\geq 2}\vb_k^\top\psp/\tn{\psp}=1/\Gamma_\beta>\min_{k\geq 2}\vb_k^\top\ps/\tn{\ps}=1/\Gamma.\nonumber
\end{align}
If not, it would imply that $\tn{\psp}=\tn{\ps}$ and that $\min_{k\geq 2}\vb_k^\top\ps=\min_{k\geq 2}\vb_k^\top\psp$. Since theorem's statement guarantees $\ps\neq\psp$, this contradicts with the unique optimality of $\psp$ when satisfying constraints $k\geq 2$ as $\ps$ would achieve the same objective.%Otherwise, it would contradict with the optimality of $\psp$ over  since 

Finally, using same argument, we also note that, $\psp$ achieves strictly less margin over $\vb_1$, namely
\begin{align}
\vb_1^\top\psp/\tn{\psp}<\vb_1^\top\ps/\tn{\ps}=1/\Gamma.\label{useful eq first}
\end{align}
If not, it would imply that $\psp$ achieves a better or equal margin at all constraints which would contradict with the optimality of $\ps$ over constraints $k\geq 1$.

Now, let us define $\pse=\eps\psp+(1-\eps)\ps$ and observe that $\pse$ also satisfies the discussion above. Namely, using $\tn{\pse}\leq \eps\tn{\psp}+(1-\eps)\tn{\ps}<\Gamma$ we find
\begin{align}
\frac{\min_{k\geq 2}\vb_k^\top\pse}{\tn{\pse}}\geq \frac{1}{\eps\tn{\psp}+(1-\eps)\tn{\ps}}>\frac{1}{\Gamma}.\label{gamt eq}%=\frac{1}{\gamt}
\end{align}
Similarly, on constraint $\vb_1$, we have that
\begin{align}
\vb_1^\top\pse/\tn{\pse}:=1/\gamp<1/\Gamma.\label{useful eq}
\end{align}
If not, it would imply that $\pse$ achieves a better or equal margin on all constraints which would contradict with the unique optimality of $\ps$ over constraints $k\geq 1$.

We will use $\gamp>\Gamma$, \eqref{useful eq}, and \eqref{gamt eq} to conclude that $\pse$ is a strictly better direction compared to a $\delta=\delta(\eps)$ neighborhood of $\psb:=\ps/\tn{\ps}$. Pick the $\delta$ (conic) neighborhood of $\ps$ such that, all $\psd$ it satisfies
\begin{align}
&\vb_k^\top\psd/\tn{\psd}\geq 1/\damp=0.5(1/\gamp+1/\Gamma)>1/\gamp\quad\text{for all}\quad k\in[K].\label{damp eq}
%&\vb_1^\top\psd/\tn{\psd}\geq1/\damp=0.5(1/\gamp+1/\Gamma)>1/\gamp.
\end{align}
In words, we choose a neighborhood with correlation profile dominated by $\pse$ (on $k=1$ and $k\geq 2$). We now lower bound the loss function over $\delta$-neighborhood and upper bound over $\pse$. Specifically, we will compare a $\psd$ within the $\delta$ neighborhood of $\ps$ with $\tn{\psd}=R$ and $\pset:=R\cdot\pseb$. To proceed, define:
\[
q^\st_i=1-\sft{\Kb_i\pset}_{\alpha_i},\quad \hat{q}_i=1-\sft{\Kb_i\psd}_{\alpha_i}
\]
Also define $q^\beta=\sft{\Kb_j\pset}_{\beta}$ which is the $j$'th softmax likelihood at token $\beta$. We will use the fact that margin at $\beta$ is small for $j$'th example to lower bound $q^\beta$ carefully. We next bound these as follows based on \eqref{useful eq}, \eqref{gamt eq}, \eqref{damp eq} (e.g.~following derivation of \eqref{smax difference})\footnote{We are essentially following identical arguments developed in the proofs of Theorem \ref{meta thm} or Theorem \ref{thm:path:joint:vp}.}
\begin{align}\label{q bounds fail}
&\log(q^\st_i)\leq -(R/\Gamma)+\log T\quad\text{for all}\quad i\neq j\\
&\log(q^\beta)\geq -(R/\gamp)-\log T\quad\text{for all}\quad i\neq j\\
&\log(q^\st_j-q^\beta)\leq -(R/\Gamma)+\log T\quad\text{for all}\quad i\neq j\\
&\log(\hat{q}_i)\leq -(R/\damp)+\log T\quad\text{for all}\quad i\in[n].
\end{align}
$\bullet$ \textbf{Lower bounding $\Lc(\psd)$:} Using the last inequality, on $\psd$ (within the $\delta$ neighborhood of $\ps$), we have the following lower bound: Set $\x^\delta_i=\X_i^\top\sft{\Kb_i\psd}$ and $M:=\sup_{i\in[n],t,\tau\in[T]}\tn{\x_{it}-\x_{i\tau}}$ and note that $\tn{\x^\delta_i-\x_{\alpha_i}}\leq M\hat{q}_i$. Also let $B$ and $A$ be the lower and upper bound of $-\ell'$ over $[-M\tn{\vb},M\tn{\vb}]$ interval. Finally, define $\Lc_\st=\frac{1}{n}\sum_{i=1}^n \ell(\vb^\top\x_{i\alpha_i})$. We find
\begin{align}\label{psd bound}
|\Lc(\psd)-\Lc_\st|&=\frac{1}{n}\sum_{i=1}^n|\ell(Y_i\cdot\vb^\top \x^\delta_i)-\ell(Y_i\cdot\vb^\top \x_{i\alpha_i})|\\
&\leq B\hat{q}_{\max} M\tn{\vb}\\
&\leq TBM\tn{\vb} e^{-R/\damp}.
\end{align}
This implies $\Lc(\psd)\geq \Lc_\st-TBM\tn{\vb} e^{-R/\damp}$.

$\bullet$ \textbf{Upper bounding $\Lc(\pset)$:} On $\pse$, we upper bound the loss as follows. Define the loss $\Lc^{-j}(\pb)=\frac{1}{n}\sum_{i\neq j}\ell(Y_i\cdot f(\X_i))$ i.e.~loss over all training data except the $j$'th one. Repeating the argument identical to \eqref{psd bound}, we find that
\[
|\Lc^{-j}(\pset)-\Lc^{-j}_\st|\leq TBM\tn{\vb} e^{-R/\Gamma}.
\]
The critical term is the $j$'th loss which we need to upper bound as follows. Set $\x^\eps_j=\X_j^\top \sft{\Kb_j\pset}$ and define the score improvement by $\beta$ to be $\bgag=Y_j\cdot\vb^\top(\x_{i\beta}-\x_{j\alpha_j})>0$. We note that
\begin{align}
Y_j\cdot\vb^\top\x^\eps_j-Y_j\cdot\vb^\top \x_{\alpha_j}&=q^\beta Y_j\cdot\vb^\top(\x_{i\beta}-\x_{\alpha_j})+\sum_{t\notin\{\alpha_j,\beta\}}  \sft{\Kb_j\pset}_{t}Y_j\cdot\vb^\top(\x_{it}-\x_{\alpha_j})\\
&\geq q^\beta\bgag-(q^\st_j-q^\beta)M\tn{\vb}\\
&\geq T^{-1}\bgag e^{-R/\gamp}-TBM\tn{\vb} e^{-R/\Gamma}.
\end{align}
Combining these into $\Lc(\pset)=\Lc^{-j}(\pset)+n^{-1}\ell(Y_j\cdot\vb^\top\x^\eps_j)$ and using $A\leq -\ell'\leq B$, we obtain the lower bound
\begin{align}
\Lc(\pset)-\Lc_\st\leq 2TBM\tn{\vb} e^{-R/\Gamma}-An^{-1}T^{-1}\bgag e^{-R/\gamp}.
\end{align}
In conclusion, we find that $\Lc(\pset)>\Lc(\psd)$ whenever
\[
An^{-1}T^{-1}\bgag e^{-R/\gamp}>2TBM\tn{\vb} (e^{-R/\Gamma}+ e^{-R/\damp}).
\]
Using the relationship $\gamp\geq \damp\geq \Gamma$ and noticing $1/\damp-1/\gamp=(1/\Gamma-1/\gamp)/2$, this is implied by
\[
e^{R(1/\damp-1/\gamp)}>4T^2nBMA^{-1}\tn{\vb}\iff R>\frac{2\gamp \Gamma}{\gamp-\Gamma}\log(4T^2nBMA^{-1}\tn{\vb}).
\]
Thus, as advertised, we found that, for any $\eps>0$, there exists $R_\eps$ such that, over the set $\cone_{\eps}(\ps)\bigcap\{\pb\bgl \tn{\pb}\geq R_\eps\}$, $\pset$ achieves smaller loss compared to $\Lc(\psd)$ for all $\psd\in \cone_{\delta}(\ps)\bigcap\{\pb\bgl \tn{\pb}\geq R_\eps\}$. This in turn implies that $\pbb(R)/R\not\rightarrow \ps$ since $\pbb(R)$ lies outside of $\cone_{\delta}(\ps)$ (a small conic/directional neighborhood around $\ps$).
\end{proof}
