# Supplementary material for: Max-Margin Token Selection in Attention Mechanism
Source: arXiv:2306.13596 source file (2023-12-08)
Supplement: Supplementary file 8 [file app_tightest_06_15.tex]

\subsection{Regularization Path Only Converges to Locally-Optimal Max Margin Directions}

\subsubsection{Supporting Lemma}

We provide a lemma below that will be helpful for streamlining our analysis. We start with a definition.
\begin{definition}[Selected-tokens, Neighbors, Margins, and Neighbor-optimality of a direction] \label{def direction stuff}Let $\qb\in\R^d-\{0\}$ and $(Y_i,\Kb_i,\X_i)_{i=1}^n$ be our dataset. Define the (possibly non-unique) selected-tokens of $\qb$ to be\footnote{If $\alpha_i$ is unique for all $i\in[n]$, let us call it, unique selected tokens.}
\[
\alpha_i\in \arg\max_{t\in[T]}\kb_{it}^\top\qb.
\]
Next define the margin and directional-neighbors for $\qb$ to be the minimum margin tokens to the selected-tokens i.e.
\[
\Gamma_{\qb}=\min_{i\in[n],t\neq\alpha_i} (\kb_{i\alpha_i}-\kb_{it})^\top\qb\quad \text{and}\quad \Mc_{\qb}=\arg\min_{i\in[n],t\neq\alpha_i} (\kb_{i\alpha_i}-\kb_{it})^\top\qb.
\]
Finally, we say that $\qb$ is neighbor-optimal if the scores of its directional-neighbors are strictly less than the corresponding selected-token. Concretely, for all $(i,t)\in \Mc_{\qb}$, we require that
\[
\bgam_{it}=\x_{it}^\top\vb<\bgam_{i\alpha_i}=\x_{i\alpha_i}^\top\vb.
\]
\end{definition}

\begin{lemma}[When does one direction dominate another?]\label{lem dominate} Suppose $\qb,\pb\in\R^d$ be two unit Euclidean norm vectors with identical selected tokens. Specifically, for each $i\in[n]$, there exists unique $\alpha_i\in[T]$ such that $\alpha_i= \arg\max_{t\in[T]}\kb_{it}^\top\qb= \arg\max_{t\in[T]}\kb_{it}^\top\pb$. Suppose directional margins obey $\Gamma_{\qb}<\Gamma_{\pb}$ and set $\delta_\Gamma=\Gamma_{\pb}-\Gamma_{\qb}$.
\begin{itemize}
\item Suppose $\qb$ and $\pb$ are both neighbor-optimal. Then, for some $R(\delta_\Gamma)$ and all $R>R(\delta_\Gamma)$, we have that $\Lc(R\cdot\pb)<\Lc(R\cdot\qb)$.
\item Suppose $\qb$ has a unique directional-neighbor and is not neighbor-optimal (i.e.~this neighbor has higher score). Let $\delta_{\qb}$ is the margin difference between unique directional-neighbor and the second minimum-margin neighbor (i.e.~the one after the unique one, see \eqref{deltaq def}) of $\qb$. Then, for some $R(\delta_\Gamma\wedge \delta_{\qb})$ and all $R>R(\delta_\Gamma\wedge \delta_{\qb})$, we have that $\Lc(R\cdot\qb)<\Lc(R\cdot\pb)$.
\end{itemize}
\end{lemma}
\begin{proof} We prove these two statements in order. First define the directional risk baseline induced by letting $R\rightarrow\infty$ and purely selecting the tokens $\bal=(\alpha_i)_{i=1}^n$. This is given by $\Lc_\st=\frac{1}{n}\sum_{i=1}^n\ell(Y_i \cdot\vb^\top\x_{i\alpha_i})$. We evaluate $\qb,\pb$ with respect to $\Lc_\st$. To proceed, let $\s_{i}=\sft{R\Kb_i\qb}$. Define $\Gamma^{it}_{\qb}=\kb_{i\alpha_i}^\top\qb-\kb_{it}^\top\qb$. Note that, the smallest value for $t\neq \alpha_i$ is achieved for $\Gamma_{\qb}$. For sufficiently large $R\gtrsim \order{1/\Gamma_{\qb}}$, observe that, for $t\neq\alpha_i$
\begin{align}
e^{-R\Gamma^{it}_{\qb}}\geq \s_{it}=\frac{e^{R\kb_{it}^\top\qb}}{\sum_{t\in [T]}e^{R\kb_{it}^\top\qb}}\geq 0.5 e^{-R\Gamma^{it}_{\qb}}.\label{up low bound}
\end{align}
Recalling the score definition and let $M_+,M_-$ be the upper and lower bounds on $-\ell'$ over its bounded domain that scores fall on. Note that, for some intermediate $M_+\geq M_i\geq M_-$ values
\begin{align}%\neq \alpha_i
\Lc(R\qb)-\Lc_\st&=\frac{1}{n}\sum_{i=1}^n \ell(\sum_{t\in [T]}\s_{it} \bgam_{it})-\ell(\bgam_{i\alpha_i})\\
&=\frac{1}{n}\sum_{i=1}^nM_i \sum_{t\neq \alpha_i}\s_{it} (\bgam_{i\alpha_i}-\bgam_{it}).
%\\&=\frac{1}{n}\sum_{i=1}^nM_i \sum_{t\neq \alpha_i}\frac{e^{-}}{} (\bgam_{i\alpha_i}-\bgam_{it}).
\end{align}
Now, using \eqref{up low bound} for a refreshed $M_+\geq M_{it}\geq 0.5M_-$ values, we can write
\begin{align}%\neq \alpha_i
\Lc(R\qb)-\Lc_\st&=\frac{1}{n}\sum_{i=1}^n \sum_{t\neq \alpha_i}M_{it}e^{-R\Gamma^{it}_{\qb}} (\bgam_{i\alpha_i}-\bgam_{it}).\label{eq so far}
\end{align}
The same bound also applies to $\pb$ with some $M'_{it},$ multipliers
\begin{align}%\neq \alpha_i
\Lc(R\pb)-\Lc_\st&=\frac{1}{n}\sum_{i=1}^n \sum_{t\neq \alpha_i}M'_{it}e^{-R\Gamma^{it}_{\pb}} (\bgam_{i\alpha_i}-\bgam_{it}).
\end{align}
We can now proceed with the proof.

\textbf{Case 1: $\qb$ and $\pb$ are both neighbor-optimal.} This means that $\bgam_{i\alpha_i}-\bgam_{it}>0$ for all $i,t\neq\alpha_i$. Let $K_+>K_->0$ be upper and lower bounds on  $\bgam_{i\alpha_i}-\bgam_{it}$ values. We can now upper bound the right hand side of \eqref{eq so far} via
\[
M_+K_+T e^{-R\Gamma_{\qb}} \geq \Lc(R\qb)-\Lc_\st\geq \frac{1}{2n}M_-K_-e^{-R\Gamma_{\qb}}.
\]
Consequently, $\Lc(R\qb)>\Lc(R\pb)$ as soon as $\frac{1}{2n}M_-K_-e^{-R\Gamma_{\qb}}>M_+K_+T e^{-R\Gamma_{\pb}}$. Since $M_+,K_+,n,T$ are global constants, this happens under the stated condition on the margin gap $\Gamma_{\pb}-\Gamma_{\qb}$.

\textbf{Case 2: $\qb$ has a unique directional-neighbor and is not neighbor-optimal.} In this scenario, $\Lc(R\qb)-\Lc_\st$ is actually negative for large $R$. To proceed, let us recall the maximum score difference $K_+=\sup_{i,t\neq\alpha_i}|\bgam_{i\alpha_i}-\bgam_{it}|$. Also let $(j,\beta)$ be the unique directional neighbor achieving the minimum margin $\Gamma_{\qb}$. Then, $\delta_\qb$ -- the margin difference between unique directional-neighbor and the second minimum-margin neighbor (i.e.~the one after the unique one) of $\qb$ -- is defined as
\begin{align}
\delta_{\qb}=\min_{i\in[n],t\neq\alpha_i,(i,t)\neq (j,\beta)} \Gamma^{it}_{\qb}-\Gamma^{j\beta}_{\qb}.\label{deltaq def}
\end{align}
To proceed, we can write
\[
\Lc(R\pb)-\Lc_\st\geq -M_+K_+T e^{-R\Gamma_{\pb}}.
\]
On the other hand, setting $\kappa=\bgam_{j\beta}-\bgam_{j\alpha_j}>0$, we can bound 
\begin{align}
\Lc(R\qb)-\Lc_\st&=-\frac{1}{n}M_{j\beta}e^{-R\Gamma_{\qb}}\kappa+ \frac{1}{n} \sum_{i\in[n],t\neq \alpha_i,(i,t)\neq (j,\beta)}M_{it}e^{-R\Gamma^{it}_{\qb}} (\bgam_{i\alpha_i}-\bgam_{it})\\
&\leq -\frac{1}{n}M_-e^{-R\Gamma_{\qb}}\kappa+ M_+K_+T e^{-R(\Gamma_{\qb}+\delta_{\qb})}.
\end{align}
Consequently, we have found that $\Lc(R\pb)>\Lc(R\qb)$ as soon as
\[
\frac{1}{n}M_-e^{-R\Gamma_{\qb}}\kappa\geq M_+K_+T (e^{-R(\Gamma_{\qb}+\delta_{\qb})}+e^{-R\Gamma_{\pb}})
\]
This happens when $R\gtrsim \frac{1}{\delta_{\qb}\wedge (\Gamma_{\pb}-\Gamma_{\qb})}$ (up to logarithmic terms) establishing the statement of the lemma.
\end{proof}

\subsubsection{Proof of Theorem \ref{tightest reg path}}
%Below, we assume that $\ps(\bal)$ exists (i.e.~SVM is solvable) for any choice of indices $\bal=(\alpha_i)_{i=1}^n$. 
Define the locally-optimal unit directions
\[
\Pc=\left\{\frac{\ps(\bal)}{\tn{\ps(\bal)}}~\big|~\bal~\text{is a locally-optimal set of indices}\right\}.
\]
The theorem below shows that cone-restricted regularization paths can only directionally converge to an element of this set.
%$\Ac$ be the set of locally optimal indices $\bal$ and $\Pc$ be the set of .
%Assume all token scores are distinct and $\ps(\bal)$ exists (i.e.~SVM is solvable) for any choice of indices $\bal=(\alpha_i)_{i=1}^n$. 
\begin{theorem}[Failure of Other Regularization Paths] \label{tightest reg path}Fix a unit Euclidean norm vector $\qb\in\R^d$ such that $\qb\not\in\Pc$. Assume that
\begin{itemize}
\item All token score differences $\bgam_{it}-\bgam_{i\tau}=Y_i\cdot \vb^\top(\x_{it}-\x_{i\tau}) $ are distinct for $i\in[n],t\neq\tau\in[T]$.\footnote{This is a simplifying assumption and holds for almost all datasets/tokens.}%for the same input $i$ 
\item $\ps(\bal)$ exists (i.e.~SVM is solvable) for any choice of indices $\bal=(\alpha_i)_{i=1}^n\subset [T]$. 
\end{itemize}
For any $\eps>0$, there exists $R_\eps>0$ as follows: Consider the conic neighborhood of $\qb$: $\Cc_{\eps}:=\Cc_{\eps}^\qb=\cone_{\eps}(\qb)\bigcap\left\{\pb~|~\tn{\pb}\geq R_\eps\right\}$. Define the local path $\pbb(R)=\min_{\pb\in \Cc_{\eps},\tn{\pb}\leq R}\Lc(\pb)$. Then $\underset{R\rightarrow\infty}{\lim}\frac{\pbb(R)}{\tn{\pbb(R)}}\neq \qb$.
\end{theorem}
\begin{proof} We will prove the result by splitting the problem into distinct cases. In all cases, we construct an alternative direction which achieves a strictly better objective than some $\delta=\delta(\eps)>0$ neighborhood of $\qb$ which demonstrates the suboptimality of the $\qb$ direction. Define this $\delta$ neighborhood to be 
\[
\Nc^R_\delta=\{\tn{\frac{\pb}{\tn{\pb}}-\qb}\leq\delta,R\geq \tn{\pb}\geq R_\eps\}.
\]
We need a few more definitions which follow Definition \ref{def direction stuff}. First, define the indices chosen by $\qb$. This is given by
\[
\alpha_i=\arg\max_{t\in[T]}\kb_{it}^\top\qb.
\]
To proceed, we first consider the scenario where $\alpha_i$ is unique for all $i\in[n]$ i.e.~$c\cdot\qb$ will choose a single token per input as we let $c\rightarrow\infty$. We will later revisit the setting when $\arg\max$ is not a singleton and $\qb$ selects multiple tokens. 

$\bullet$ \textbf{(A) $\qb$ selects single token per input:} Now that indices $\bal=(\alpha_i)_{i=1}^n$ are uniquely determined, we know that $\qb$ direction eventually selects tokens $\kb_{i\alpha_i}$. Define the margin 
\[
\Gamma_{\qb}=\min_{i\in[n]}\min_{t\neq\alpha_i}(\kb_{i\alpha_i}-\kb_{it})^\top\qb.
\] 
Secondly, recall the set of directional-neighbors defined as the indices that achieve $\Gamma_{\qb}$. Namely, these are the coordinates $(i,t)$ such that
\[
\Mc_\qb=\{(i,t)~\big|~(\kb_{i\alpha_i}-\kb_{it})^\top\qb=\Gamma_{\qb}\}.
\]
Also, let us call $\qb$ \emph{neighbor-optimal} if $\bgam_{it}<\bgam_{i\alpha_i}$ for all $(i,t)\in \Mc_\qb$.

We will split this scenario into two cases: $\bal$ is neighbor-optimal vs $\bal$ is not neighbor-optimal.

$\diamond$ \textbf{(A1) $\bal$ is neighbor-optimal.} In this case, we will argue that max-margin direction $\psb:=\ps(\bal)/\tn{\ps(\bal)}$ can be used to construct a strictly better objective than $\qb$. Specifically, consider the direction $\qb'=\frac{\qb+\eps\psb}{\tn{\qb+\eps\psb}}$. Observe that, $\qb'$ lies within $\cone_{2\eps}(\qb)$,\footnote{As a result, let us prove the result for $\eps\gets 2\eps$ without losing generality.}
\[
\qb^\top \qb'\geq \frac{1-\eps}{1+\eps}\geq 1-2\eps.
\]
 We now argue that, there exists $\delta=\delta_\eps>0$ such that for all $R>R_\eps$
\begin{align}
\Lc(R\cdot\qb')< \min_{\pb\in \Nc^R_{\delta}}\Lc(\pb).\label{desired delta bound}
\end{align}
To prove this, we study the margin $\Gamma_{\qb'}$ induced by $\qb'$ and the maximum margin $\Gamma_\delta$ induced within $\pb\in \Nc^R_{\delta}$. Concretely, we will show that $\Gamma_{\qb'}>\Gamma_{\delta}$ and directly apply the first statement of Lemma \ref{lem dominate} to conclude with \eqref{desired delta bound}.

Let $\Gamma=1/\tn{\ps(\bal)}$ be the margin induced by $\psb$. Note that $\Gamma>\Gamma_{\qb}$ by the optimality of $\ps(\bal)$ and the fact that $\qb\neq \ps(\bal)$. Consequently, we can lower and upper bound the margins via
\begin{align}
\Gamma_{\qb'}&=\min_{i\in[n]}\min_{t\neq\alpha_i}(\kb_{i\alpha_i}-\kb_{it})^\top\qb'\geq \frac{\Gamma_\qb+\eps\Gamma}{1+\eps}\geq \Gamma_\qb+\frac{\eps}{2}(\Gamma-\Gamma_\qb)\\
\Gamma_\delta&=\max_{\pb\in \Nc^R_{\delta}}\min_{i\in[n]}\min_{t\neq\alpha_i}(\kb_{i\alpha_i}-\kb_{it})^\top\pb/\tn{\pb}\\
&\leq \max_{\tn{\rb}\leq 1}\min_{i\in[n]}\min_{t\neq\alpha_i}(\kb_{i\alpha_i}-\kb_{it})^\top(\qb+\delta\rb)\\
&\leq \Gamma_\qb+M\delta,
\end{align}
where $M=\max_{i,t,\tau}\tn{\kb_{it}-\kb_{i\tau}}$. Consequently, setting $\delta=\frac{\eps}{4M}(\Gamma-\Gamma_\qb)$, we find that
\[
\Gamma_{\qb'}\geq\Gamma_\delta+\frac{\eps}{4}(\Gamma-\Gamma_\qb).
\]
Equipped with this inequality, we apply the first statement of Lemma \ref{lem dominate} which concludes that\footnote{Here, we apply this lemma to compare $\qb'$ against all $\pb\in\Nc_{\delta}^R$. We can do this uniform comparison because the $R$ requirement in Lemma \ref{lem dominate} only depends on the margin difference and global problem variables and not the particular choice of $\pb\in\Nc_{\delta}^R$.} for some $R_0=R(\frac{\eps}{4}(\Gamma-\Gamma_\qb))$ and all $R>R_0$, \eqref{desired delta bound} holds. This in turn implies that, within $\Cc_{\eps}^{\qb}$, the optimal solution is at least $\delta=\delta(\eps)>0$ away (in terms of $\ell_2$-normalized distance) proving that $\underset{R\rightarrow\infty}{\lim}\frac{\pbb(R)}{\tn{\pbb(R)}}\neq \qb$.

%\begin{lemma}
%\end{lemma}
%\begin{proof}
%\end{proof}

%s within each input $i\in[n]$ are unique
$\diamond$ \textbf{(A2) $\bal$ is not neighbor-optimal.} In this scenario, we construct a direction towards a directional neighbor of $\bal$ which is strictly better scorewise. Concretely, recall that $\Mc_\qb$ is the set of directional neighbors and that score differences of the token pairs are unique. Choose the (unique) index $(j,\beta)\in \Mc_{\qb}$ as follows
\[
(j,\beta)=\arg\min_{(i,t)\in\Mc_{\qb}} \bgam_{i\alpha_i}-\bgam_{it}.
\]
% Analysis of the scenario where selected-tokens change is essentially same as Setting (B) ``$\qb$ selects multiple tokens'' below. 
%\frac{\qb+\eps\qb^\perp}{\tn{\qb+\eps\qb^\perp}}$
In words, we are seeking for the neighbor with the highest relative score compared to the selected direction. Now that we chose this neighbor, define the score difference $\kappa=\bgam_{j\beta}-\bgam_{j\alpha_j}>0$. We know $\kappa>0$ because $\bal$ is not neighbor optimal. To proceed, we choose a perturbation direction $\qb^\perp=\frac{\kb_{j\alpha_j}-\kb_{j\beta}}{\tn{\kb_{j\alpha_j}-\kb_{j\beta}}}$.  We now investigate the candidate $\qb'=\qb+\eps\qb^\perp$ and compare against $\Nc^R_\delta$ to establish \eqref{desired delta bound}. We assume that neighborhood $\eps$ is small enough so that selected-tokens $\bal$ remain unchanged within $\Cc_\eps$. This is without generality because if directional convergence fails in a small neighborhood of $\qb$, it will fail in a larger neighborhood. %Now, since $\kb_{it}-\kb_{i\tau}$ are all linearly independent

%Suppose $\qb^\perp$ achieve a margin of $\Gamma^\perp$ and set $M_\eps=\tn{\qb+\eps\qb^\perp}$. 
Let $K=\max_{i,t,\tau}\tn{\kb_{it}-\kb_{i\tau}}$. We again proceed with a margin analysis so that we can apply Lemma \ref{lem dominate}:

% Define $\bal'=(\alpha'_i)_{i=1}^n$ where $\alpha'_i=\alpha_i$ for all $i\neq j$ and $\alpha'_j=\beta$. Set $\qb^\perp=\ps(\bal')/\tn{\ps(\bal')}$ and
\begin{enumerate}
\item For token $(j,\beta)$, we have that %(Use the optimality of $\qb$, NOPE: Just use linear independence of $\kb_{it}-\kb_{i\tau}$ pairs)%$\qb^\perp$
\[
(\kb_{j\alpha_j}-\kb_{j\beta})\qb'=(\kb_{j\alpha_j}-\kb_{j\beta})(\qb+\eps\qb^\perp)\leq \Gamma_{\qb}-\eps \tn{\kb_{j\alpha_j}-\kb_{j\beta}}.
\]
\item For all other tokens $(i,t)$ with $t\neq \alpha_i$, we have that
\[
(\kb_{i\alpha_i}-\kb_{it})\qb'=(\kb_{i\alpha_i}-\kb_{it})\frac{\qb+\eps\qb^\perp}{M_\eps}\geq M_\eps^{-1}(\Gamma_{\qb}+\eps \Gamma^\perp).
\]
\end{enumerate}

\begin{comment}
\newpage
 Specifically, we will apply the second statement of Lemma \ref{lem dominate} via the following intermediate results:
%upper bounded by a $\qb$ and dataset-dependent constant
\begin{itemize}
\item \textbf{Result 1:} 
\item \textbf{Result 2:} 
\item \textbf{Result 3:} 
\end{itemize}

% via the following SVM sconsider the perturbation direction obtained by maximizing the margin of $(j,\beta)$ namely $\pb^\perp=\kb_{j\beta}-\kb_{j\alpha_j}$.

%solving the following SVM that maximizes the margin of $(j,\beta)$, namely
%\begin{align*}
%\pb^\perp=\min\tn{\pb}\quad\text{such that}\quad \pb^\top (\kb_{i\alpha_i}-\kb_{it})
%\end{align*}

%indices $(i_k,t_k)_{k=1}^K\subset \Mc_{\qb}$ be those that achieve highest

$\bullet$ \textbf{(B) $\qb$ selects multiple tokens for some inputs:}
\end{comment}
\end{proof}
