# Supplementary material for: Max-Margin Token Selection in Attention Mechanism
Source: arXiv:2306.13596 source file (2023-12-08)
Supplement: Supplementary file 12 [file bc_app_GD_2.tex]

\section{Proofs on Gradient Descent}\label{app:conv:gd}
\subsection{Descent and Gradient Correlation Conditions}
The lemma below identifies conditions under which $\pso$ is a global descent direction for $\Lc(\pb)$.
\begin{lemma}[Global descent conditions]\label{global des lem} Suppose $\ell(\cdot)$ is a strictly decreasing loss function and either of the following two conditions holds
\begin{itemize}
\item \textbf{Scores of non-optimal tokens are same:} For all $i\in[n]$ and $t_1,t_2\neq \op_i$, $\vb^\top \x_{it_1}=\vb^\top \x_{it_1}$.
\item \textbf{All tokens are support vectors:} Consider \eqref{attnsvm} with optimal indices $(\op_i)_{i=1}^n$. $(\kbo_i-\kb_{it})^\top\pso=1$ for all $t\neq \op_i,i\in[n]$.
\end{itemize}
Define 
\begin{itemize}
    \item $\abg^i:=1=\inf_{t\neq \op_i} (\kbo_i-\kb_{it})^\top\pso$,
    \item $\bgag^i=\inf_{t\neq \op_i} Y_i\cdot(\x^\op_i-\x_{it})^\top\vb$,
    \item $\lgt_i=p_{\op}(1-p_{\op})$ where $p_{\op}=\sft{\Kb_i\pb}_{\op_i}$,
    \item $\ell'_i=\ell'(Y_i\cdot \vb^\top \X_i^\top\sft{\Kb_i\pb})<0$.
    %\item $\Lc(\pb)=\bgam^\top \sft{\ab}=\bgam_1\sft{\ab}_1+\gamma(1-\sft{\ab}_1)$.
    %\item Q: $\sft{\ab}_1+\sft{\ab'}_1>2\sft{\frac{\ab+\ab'}{2}}_1$.
\end{itemize}
Then, for all $\pb\in\R^d$, the training loss \eqref{lin det los} obeys 
\[
-\li\nabla\Lc(\pb),\pso\ri\geq \min_{i\in [n]} \left\{-\ell'_i\cdot\lgt_i\cdot\abg^i\cdot\bgag^i\right\}> 0.
\]
\end{lemma}
\begin{proof} In order to show this result, let us recall the gradient evaluated at $\pb$ which is given by 
\[\nabla\Lc(\pb)=\frac{1}{n}\sum_{i=1}^n \ell'_i\cdot\Kb_i^\top \sfp{\ab_i}\bgam_i.\] Here $\bgam_i=Y_i\cdot X_i\vb$, $\ab_i=\Kb_i\pb$, and $\ell'_i=\ell'(Y_i\cdot \vb^\top \X_i^\top\sft{\Kb_i\pb})$. Set $\abm_i=\Kb_i\pso$ to obtain
\begin{align}\label{grad def}
\li\nabla\Lc(\pb),\pso\ri&=\frac{1}{n}\sum_{i=1}^n\ell'_i\cdot\li\abm_i,\sfp{\ab_i}\bgam_i\ri.
%\\&=\frac{1}{n}\sum_{i=1}^n\li\abm_i,\sfp{\ab_i}\bgam_i\ri
\end{align}
To proceed, we will prove that individual summands are all strictly negative. To show that, without losing generality, let us focus on the first input and drop the subscript $i$ for cleaner notation. This yields
\begin{align}
\li\abm,\sfp{\ab}\bgam\ri&=\abm^\top\diag{\sft{\ab}}\bgam-\abm^\top\sft{\ab}\sft{\ab}^\top\bgam.
%\\&=%\frac{\sum_{t=1}^T \abm_t\bgam_t e^{\ab_t}}{\sum_{\tau=1}^T e^{\ab_\tau}}
\end{align}
Without losing generality, assume optimal token is the first one. The lemma has two scenarios. In the first scenario (same non-optimal scores), $\bgam_t$ is a constant for all $t\geq 2$. In the second scenario (all tokens are support), $\abm_t=\kb_t\pso$ is constant for all $t\geq 2$. Since $\abm,\bgam$ vectors are represented symmetrically in the gradient correlation, verifying these two conditions are equivalent. 

To proceed, we will prove the following (focusing on the first condition): Suppose $\gamma=\bgam_{t\geq 2}$ is constant, $\bgam_1,\abm_1$ are the largest indices of $\bgam,\abm$. Then, for any $\s$ obeying $\sum_{t\in[T]}\s_t=1,\s_t\geq 0$, we have that $\abm^\top\diag{\s}\bgam-\abm^\top\s\s^\top\bgam>0$. To see this, we write
\begin{align}
\abm^\top\diag{\s}\bgam-\abm^\top\s\s^\top\bgam&=\sum_{t=1}^T \abm_t\bgam_t\s_t-\sum_{t=1}^T \abm_t\s_t\sum_{t=1}^T \bgam_t\s_t\label{grad def2}\\
&=(\abm_1\bgam_1\s_1+\gamma\sum_{t\geq 2}\abm_t\s_t)-(\bgam_1\s_1+\gamma(1-\s_1))(\abm_1\s_1+\sum_{t\geq 2}^T \abm_t\s_t)\\
&=\abm_1(\bgam_1-\gamma)\s_1(1-\s_1)+(\gamma-(\bgam_1\s_1+\gamma(1-\s_1)))\sum_{t\geq 2}^T \abm_t\s_t\\
&=\abm_1(\bgam_1-\gamma)\s_1(1-\s_1)-(\bgam_1-\gamma)\s_1\sum_{t\geq 2}^T \abm_t\s_t\\
&=(\bgam_1-\gamma)(1-\s_1)\s_1[\abm_1-\frac{\sum_{t\geq 2}^T \abm_t\s_t}{\sum_{t\geq 2}\s_t}].
\end{align}
% Assume $R$ is large enough.
% Case 1: If $\pso\approx\pb_t$ and $\abm\approx \ab_t$, then the difference of the gradient correlations are already small as $a_1-a_{t\geq 2}$ are constant, same, and support vecs have dominating probability over rest.
% Case 2: If $\pso-\pb_t$ large, then nearest token will dominate the term and result in bad outcome for $\pb_t$. Because the token that is nearest will have dominating probability but will also achieve the smallest margin.
To proceed, recall the definitions $\bgag=\bgam_1-\max_{t\geq 2}\bgam_t$ and $\abg=\abm_1-\max_{t\geq 2}\ab_t$. With these, we obtain
\[
\abm^\top\diag{\s}\bgam-\abm^\top\s\s^\top\bgam\geq \abg \bgag \s_1(1-\s_1),
\]
which is the advertised result after noticing $\s_1(1-\s_1)$ is the logistic derivative and infimum'ing over all inputs and multiplying by $\ell'_i$.
\end{proof}

\begin{assumption} [\neis have same score]\label{assum:regular} Fix token indices $\bal=(\alpha_i)_{i=1}^n$ and let $\Tc_i\subset[T]$ be their \neis for $i\in[n]$. For all $i\in[n]$ and $t_1,t_2\in\Tc_i$, $\kb_{it_1}^\top\ps=\kb_{it_1}^\top \ps$.
% Relaxing this assumption is tricky because there are $\pb$ directions with gradients subpar correlations with $\ps$. The reason is that $\pb$ can select the lowest score neighbor to get high-corr whereas $\ps$ will be $\Omega(1)$ less corr.
\end{assumption}
\begin{lemma}[Local Gradient Condition]\label{local cond} Let $\bal=(\alpha_i)_{i=1}^n$ be locally-optimal tokens per Definition \ref{def loc opt} and suppose Assumption \ref{assum:regular} holds. There exists a scalar $\mu=\mu(\bal)>0$  as follows: Define the set $\cone_{\mu,R}(\ps)$ to be vectors obeying $\corr{\pb,\ps}\geq 1-\mu$ and $\tn{\pb}\geq R$. 
\begin{itemize}
  \item For sufficiently large $R$, there is no local minima within $\cone_{\mu,R}(\ps)$. 
  \item Denote $\pbb=\pb/\tn{\pb}$. For any $\pi$, there exists $R_\pi$ such that all $\pb\in \cone_{\mu,R_{\pi}}(\ps)$ with obeys
\[
\li\nabla\Lc(\pb),\pbb\ri\geq (1+\pi)\li\nabla\Lc(\pb),\ps\ri,
\]
\end{itemize}
\end{lemma}
\red{[TO BE PROVEN:] As a consequence of this lemma, choosing $\pi\leq \mu/3$, gradient iterations starting within $\cone_{\mu,R_{\pi}}(\ps)$ eventually obeys $\pb\in \cone_{\mu/2,R_{\pi}}(\ps)$.}

\begin{proof} Let $\ps=\ps(\bal)$ be the solution of \eqref{attnsvm}. Define $\Cc_\mu=\{\pb\in\R^d~\big|~\corr{\pb,\ps}\geq 1-\mu\}$. Let $(\Tc_i)_{i=1}^n$ be the set of all \neis per Definition \ref{def loc opt}. Let $\Tcb_i=[T]-\Tc_i-\{\alpha_i\}$ be the non-SVM-neighbor tokens. Since $\ps$ is the max-margin model, we can find $\mu>0$ such that, for some $\delta>0$, for all $i\in[n], t\in\Tc_i,\tau\in\Tcb_i$, the following inequalities hold for all $\pb\in \Cc_\mu,~\tn{\pb}=\tn{\ps}=1/\Theta$ and all $i\in[n]$:
\begin{align}\label{cone-non-nei}
(\kb_{it}-\kb_{i\tau})^\top \pb&\geq \delta>0,\\%\quad\text{for all}\quad \\
(\kb_{i\alpha_i}-\kb_{i\tau})^\top \pb&\geq 1+\delta.
\end{align}
Note that such a $(\mu,\delta)$ is guaranteed to exist because \neis achieve strictly higher correlations to $\ps$ than non-neighbors which will persist around a neighborhood of $\ps$ as well.

Now that the choice of $\mu$ is determined, we need to prove the main claims. We first show that there is no local minima above some $R>0$. To see this, we write the gradient following \eqref{grad def} and \eqref{grad def2}
\begin{align}\label{grad def3}
\li\nabla\Lc(\pb),\ps\ri&=\frac{1}{n}\sum_{i=1}^n\ell'_i\cdot\li\abm_i,\sfp{\ab_i}\bgam_i\ri.
\end{align}
%(\kb_{i\alpha_i}-\kb_{i\tau})^\top \pb=
where we denoted $\ell'_i=\ell'(Y_i\cdot \vb^\top \X_i^\top\sft{\Kb_i\pb})$, $\abm_i=\Kb_i\ps$, $\ab_i=\Kb_i\pb$ and $\s_i=\sft{\ab_i}$. Using \eqref{cone-non-nei}, for non-neighbors $t\in\Tc_i,\tau\in \Tcb_i$, $\ab_{i\alpha_i}-\ab_{i\tau}\geq R\Theta(1+\delta),~\ab_{it}-\ab_{i\tau}\geq R\Theta\delta$ for $\pb\in \cone_{\mu,R}(\ps)$. Consequently, we can bound the non-neighbor softmax probabilities $\s_i=\sft{\Kb_i\pb}$ as follows
\begin{align}
Q_i=\sum_{\tau\in\Tcb_i}\s_{i\tau} \leq T e^{-R\Theta\delta}(\s_{i\alpha_i}\wedge e^{-R\Theta}\s_{i\alpha_i}).
\end{align}
%(over all $i,t$) 
Let $\gamb_i=Y_i\cdot\vb^\top \x_{it}$ be the identical score over the SVM-neighbors $t\in\Tc_i$ (per Assumption \ref{assum:regular}). Define the global constants $\Gamma=\max_{i,t\in\Tcb_i}|\bgam_{it}-\gamb_i|,A=\max_{i,t\in[T]}|\abm_{it}|$ where $\abm_i=\Kb_i\ps$.

Let us focus on a fixed datapoint $i\in[n]$, assume (without losing generality)$\alpha:=\alpha_i=1$, and drop subscripts $i$, that is,~$\alpha:=\alpha_i$, $\X:=\X_i$, $Y:=Y_i$, $\Kb:=\Kb_i$, $\abm=\Kb\ps$, $\ab=\Kb\pb$, $\s=\sft{\ab}$, $\bgam=Y\cdot\X\vb$. 
%Let $\Tc'=\Tc_i\cup\{\alpha_i\}$. Let $\s'=\sft{\ab_{\Tc'}}\in\R^{|\Tc'|}$ be the softmax probabilities induced by $\Tc'$. 
% , that is, $\gamb=\vb^\top \x_{it}$ for $t\in\Tc_i$
Over $t\in\Tcb$, we write $\bgam_t=\bgam_t-\gamb+\gamb$ to write the decompositions
\begin{align}
\sum_{t=1}^T \abm_t\bgam_t\s_t&\geq \abm_1\bgam_1\s_1+\gamb\sum_{t\geq 2}\abm_t\s_t-Q\Gamma A\\
(\bgam_1\s_1+\gamb(1-\s_1))-Q\Gamma\leq \sum_{t=1}^T \bgam_t\s_t&\leq (\bgam_1\s_1+\gamb(1-\s_1))+Q\Gamma
\end{align}

To proceed, we will show $\li\abm_i,\sfp{\ab_i}\bgam_i\ri>0$ to conclude that $\nabla \Lc(\pb)\neq 0$ in \eqref{grad def3}. Observing $|\sum_{t=1}^T \abm_t\s_t|\leq A$, we can write the correlation to $\abm$ as follows
\begin{align} 
\abm^\top\diag{\s}\bgam-\abm^\top\s\s^\top\bgam&=\sum_{t=1}^T \abm_t\bgam_t\s_t-\sum_{t=1}^T \abm_t\s_t\sum_{t=1}^T \bgam_t\s_t\label{grad def local}\\
&\geq (\abm_1\bgam_1\s_1+\gamb\sum_{t\geq 2}\abm_t\s_t-Q\Gamma A)-(\bgam_1\s_1+\gamb(1-\s_1))(\abm_1\s_1+\sum_{t\geq 2}^T \abm_t\s_t)-Q\Gamma A\\
&=\abm_1(\bgam_1-\gamb)\s_1(1-\s_1)+(\gamb-(\bgam_1\s_1+\gamb(1-\s_1)))\sum_{t\geq 2}^T \abm_t\s_t-2Q\Gamma A\\
&=\abm_1(\bgam_1-\gamb)\s_1(1-\s_1)-(\bgam_1-\gamb)\s_1\sum_{t\geq 2}^T \abm_t\s_t-2Q\Gamma A\\
&=(\bgam_1-\gamb)(1-\s_1)\s_1[\abm_1-\frac{\sum_{t\geq 2}^T \abm_t\s_t}{\sum_{t\geq 2}\s_t}]-2Q\Gamma A\\
&\geq \bgag (1-\s_1)\s_1-2Q\Gamma A.
\end{align}
where we used $\bgag=\bgam_1-\gamb$, $\abm_1-\frac{\sum_{t\geq 2}^T \abm_t\s_t}{\sum_{t\geq 2}\s_t}\geq \abg=1$.

\smallskip\smallskip\smallskip
\begin{align} 
\abm^\top\diag{\s}\bgam-\abm^\top\s\s^\top\bgam&=\sum_{t=1}^T \abm_t\bgam_t\s_t-\sum_{t=1}^T \abm_t\s_t\sum_{t=1}^T \bgam_t\s_t\label{grad def local2}\\
&=(\abm_1\bgam_1\s_1+\gamb\sum_{t\geq 2}\abm_t\s_t)-(\bgam_1\s_1+\gamb(1-\s_1))(\abm_1\s_1+\sum_{t\geq 2}^T \abm_t\s_t)\\
&=\abm_1(\bgam_1-\gamb)\s_1(1-\s_1)+(\gamb-(\bgam_1\s_1+\gamb(1-\s_1)))\sum_{t\geq 2}^T \abm_t\s_t\\
&=\abm_1(\bgam_1-\gamb)\s_1(1-\s_1)-(\bgam_1-\gamb)\s_1\sum_{t\geq 2}^T \abm_t\s_t\\
&=\frac{(\bgam_1-\gamb)}{1-\s_1}\s_1[\abm_1-\frac{\sum_{t\geq 2}^T \abm_t\s_t}{\sum_{t\geq 2}\s_t}].
\end{align}

Fix $\pi>0$ and $R=R_\pi$ is to be determined. We first show that, for sufficiently large $R$, there exists a vector $\pt$ that is arbitrarily close to $\ps$ and achieves near-optimal risk. We will prove the result for Assumption \ref{ass regular}, Case 2. The proof of Case 1 follows same argument but we can simply set $\pt=\ps$.% (rather than the additional argument). % which simplifies the argument

Recall definitions of $\qb$ and $(\tau_i)_{i=1}^n$ from Assumption \ref{ass regular} and set $\pt=\ps+\eps \qb$ for sufficiently small $\eps>0$ that will be chosen according to $\pi$. This choice ensures that $\tau_i$ is the second highest scoring token besides $\alpha_i$, that is, $\kb_{\tau_i}^\top \pt=\max_{t\neq \alpha_i} \kb_{it}^\top \pt$. Consequently, for sufficiently large $R=R(\eps)$, we obtain
\[
\]
\end{proof}
\newpage

%Assume that support neighbors of $\alpha_i$ are strictly \irel. associated 
\begin{lemma}[Gradient correlation conditions]\label{lem:gd:corr} Fix indices $\bal=(\alpha_{i=1}^n)$ and let $\ps=\ps(\bal)$ be the SVM solution separating $\alpha_i$ from remaining tokens of input $\X_i$ for $i\in[n]$. Suppose for all $i\in[n]$ and $t_1,t_2\neq \alpha_i$, $\vb^\top \x_{it_1}=\vb^\top \x_{it_1}<\vb^\top \x_{i\alpha_i}$ \red{[SO: We should actually only need this condition on the neighbor tokens, not all tokens]} and $\ell(\cdot)$ is strictly decreasing.% loss function. 
%Fix $\alpha,R>0$ and consider the set $\pb\in\R^d$ satisfying
%\[\tn{\pb}\geq R,\quad \corr{\pb,\ps}\geq \alpha,\]
%where $\corr{\cdot,\cdot}$ denotes the Pearson correlation coefficient. 

\noindent Let $\pbb=\tn{\ps}\pb/\tn{\pb}$. $M=\sup_{i,t}\tn{\kb_i}$ and $\Gamma=1/\tn{\ps}$. There exists a non-decreasing function $\delta(\cdot):\R^+\rightarrow\R^+$ such that, for any $\tn{\pb}\geq R$, we have
%Fix $R>0$ and consider the set $\tn{\pb}\geq R$. we have %Setting $\pi:=F(\alpha,R)$, we have that
\[
\li\nabla\Lc(\pb),\pbb\ri\geq (1+\pi)\li\nabla\Lc(\pb),\ps\ri.
\]
with $\pi=\min_{\eps>0} 2M(\eps+T\Gamma^{-1}e^{-\Gamma R\delta(\eps)})-\delta(\eps)$.
%where $\pi=\cdot$.
\end{lemma}
Above, observe that as $R\rightarrow \infty$, $e^{-\Gamma R\delta(\eps)}\rightarrow 0$, thus we eventually get to set $\pi=\eps=0$.

\begin{proof} The proof is similar to Lemma \ref{global des lem} at a high-level. However, we also need to account for the impact of $\pb$ besides $\ps$ in the gradient correlation. The main goal is showing that $\ps$ is the near-optimal descent direction, thus, $\pb$ cannot significantly outperform it.

To proceed, set $\s_i=\sft{\Kb_i\pb}$, $\ab_i=\Kb_i\pbb$, $\abm_i=\Kb_i\ps$. Without losing generality assume $\alpha_i=1$ for all $i\in[n]$. Set $\lgt_i=\s_{i1}/(1-\s_{i1})$. Repeating the proof of Lemma \ref{global des lem} yields
\begin{align}
\li\nabla\Lc(\pb),\ps\ri&=\frac{1}{n}\sum_{i=1}^n \ell'_i\cdot\lgt_i\cdot(\bgam_{i1}-\gamma_i)\left[\abm_{i1}-\frac{\sum_{t\geq 2}^T \abm_{it}\s_{it}}{\sum_{t\geq 2}\s_{it}}\right]\\
\li\nabla\Lc(\pb),\pbb\ri&=\frac{1}{n}\sum_{i=1}^n \ell'_i\cdot\lgt_i\cdot(\bgam_{i1}-\gamma_i)\left[\ab_{i1}-\frac{\sum_{t\geq 2}^T \ab_{it}\s_{it}}{\sum_{t\geq 2}\s_{it}}\right]
\end{align}
Focusing on a single example $i\in[n]$ with $\s,\ab,\abm$ vectors (dropping subscript $i$), for a proper choice of $\pi$, we wish to show that
\[
\left[\ab_{1}-\frac{\sum_{t\geq 2}^T \ab_{t}\s_{t}}{\sum_{t\geq 2}\s_{t}}\right]\leq (1+\pi)\cdot \left[\abm_{1}-\frac{\sum_{t\geq 2}^T \abm_{t}\s_{t}}{\sum_{t\geq 2}\s_{t}}\right].
\]

We consider two scenarios characterized by a variable $\eps$ to be determined.

\noindent\textbf{Scenario 1:} $\tn{\pbb-\ps}\leq \eps$ for some $\eps>0$. Let $M=\max_{i\in[n],t\in[T]}\tn{\kb_{it}}$. In this scenario, for any token, we find that
\[
|\ab_t-\abm_t|=|\kb_t^\top(\pbb-\ps)|\leq M\tn{\pbb-\ps}\leq M\eps.
\]
Consequently, we obtain
\[
\abm_{1}-\frac{\sum_{t\geq 2}^T \abm_{t}\s_{t}}{\sum_{t\geq 2}\s_{t}}\geq \ab_{1}-\frac{\sum_{t\geq 2}^T \ab_{t}\s_{t}}{\sum_{t\geq 2}\s_{t}}-2M\eps.
\]
Also noticing $\abm_{1}-\frac{\sum_{t\geq 2}^T \abm_{t}\s_{t}}{\sum_{t\geq 2}\s_{t}}\geq 1=\abg$, this implies that we can pick $\pi=2M\eps/\abg=2M\eps$.

\noindent\textbf{Scenario 2:} $\tn{\pbb-\ps}\geq \eps$. In this scenario, for some $\delta=\delta(\eps)$ and $\tau\geq 2$, we have that $\pb^\top (\kb_1-\kb_\tau)=\ab_1-\ab_\tau\leq 1-2\delta$. Here $\tau=\arg\max_{\tau\geq 2}\pb^\top \kb_\tau$ denotes the nearest point to $\kb_1$. Recall that $\s=\sft{\RR\ab}$ where $\RR=R/\tn{\ps}$. To proceed, split the tokens into two groups: Let $\Nc$ be the group of tokens obeying $\pb^\top (\kb_1-\kb_\tau)\leq 1-\delta$ and $[T]-\Nc$ be the rest.

Observe that
\[
\frac{\sum_{t\in \Nc}\s_t}{\sum_{t\geq 2}\s_t}\leq\frac{\sum_{t\in \Nc}\s_t}{\sum_{t=\tau}\s_t}\leq  T\frac{e^{\delta \RR}}{e^{2\delta\RR}}=Te^{-\RR\delta}.
\]
Plugging this in, we obtain
\[
\frac{\sum_{t\geq 2}^T (\ab_1-\ab_{t})\s_{t}}{\sum_{t\geq 2}\s_{t}}=\frac{\sum_{t\in\Nc}^T (\ab_1-\ab_{t})\s_{t}}{\sum_{t\geq 2}\s_{t}}+\frac{\sum_{t\in[T]-\Nc}^T (\ab_1-\ab_{t})\s_{t}}{\sum_{t\geq 2}\s_{t}}\leq (1-\delta)(1-Te^{-\RR\delta})+2\Gamma^{-1}MTe^{-\RR\delta}.
\]
Using the fact that $\abg\geq 1$, this allows for the choice $\pi=2MT\Gamma^{-1}e^{-\RR\delta}-\delta$. Combining the two scenarios and optimizing over the choice of $\eps>0$ (which is a free variable), we obtain the upper bound of 
\[
\pi = \min_{\eps>0}2M\eps\vee (2MT\Gamma^{-1}e^{-\Gamma R\delta(\eps)}-\delta(\eps))=\min_{\eps>0} 2M(\eps+T\Gamma^{-1}e^{-\Gamma R\delta(\eps)})-\delta(\eps).
\]
\end{proof}
